# Supplementary material for: A survey of stellar X-ray flares from the XMM-Newton serendipitous source catalogue: Hipparcos-Tycho cool stars
Source: arXiv:1506.05289 ancillary file (2015-06-17)
Supplement: Supplementary file 1 [file Table-C.1-StarsObs-ElOnly-v02.pdf]

| DETID | Star_Name                | Alt_Name                | Tycld        | Vmag | B-V  | Star_SpType | Star_Type           | Dist | DistRef | OBS_TARGET | CoolVflag | SRCID | SrcIdOther | IAUNAME               | logFxFv | logLx |
|-------|--------------------------|-------------------------|--------------|------|------|-------------|---------------------|------|---------|------------|-----------|-------|------------|-----------------------|---------|-------|
| 1916  | UY Scl                   |                         | 7524 00154 1 | 12.2 | 1.0  |             | W UMa               | 137  | HIP     | FALSE      | TRUE      | 1821  |            | 2XMM J001445.7-391435 | -2.0    | 30.0  |
| 2236  | HD 1165                  |                         | 4504 00031 1 | 8.9  | 0.8  | K0          |                     | 33   | HIP     | FALSE      | TRUE      | 2107  |            | 2XMM J001651.4+813948 | -3.6    | 28.5  |
| 15656 | HD 8191                  |                         | 9142 02608 1 | 10.4 | 0.7  | G0/G1 IV/V  |                     | 36   | N2K     | FALSE      | TRUE      | 12024 |            | 2XMM J011837.6-732526 | -2.6    | 29.0  |
| 22001 | 47 Cas B                 | HD 12230 B              | 4499 02252 1 | 5.3  | 0.3  | G0-2 V      |                     | 33   | HIP     | TRUE       | TRUE      | 17021 |            | 2XMM J020506.9+771651 | -3.1    | 30.4  |
| 23485 | HD 14716                 |                         | 9150 00224 1 | 9.6  | 0.5  | F5 V        |                     | 62   | N2K     | FALSE      | TRUE      | 18148 |            | 2XMM J021603.5-735043 | -3.1    | 29.2  |
| 30805 | CC Eri                   | HD 16157                | 7558 00585 1 | 9.1  | 1.3  | K7 V        | BY Dra              | 12   | HIP     | TRUE       | TRUE      | 24119 |            | 2XMM J023422.5-434748 | -1.5    | 29.6  |
| 32470 | CD-53 544                | 2MASS J02414683-5259523 | 8491 00656 1 | 10.6 | 1.2  | K6 Ve       | PMS                 | 28   | Z04     | TRUE       | TRUE      | 25472 |            | 2XMM J024146.8-525951 | -1.4    | 29.9  |
| 33241 | RZ Cas                   | HD 17138                | 4317 01793 1 | 6.3  | 0.1  | A3 Vv+...   | Algol               | 65   | HIP     | TRUE       | TRUE      | 26140 |            | 2XMM J024855.5+693803 | -3.3    | 30.4  |
| 37553 | kap01 Cet                | HD 20630                | 0059 01947 1 | 5.0  | 0.6  | G5 Vb       | BY Dra              | 9    | HIP     | TRUE       | TRUE      | 29517 |            | 2XMM J031921.5+032212 | -3.6    | 28.9  |
| 40682 | eps Eri                  | HD 22049                | 5296 01533 1 | 3.9  | 0.9  | K2 Vb:      | BY Dra              | 3    | HIP     | TRUE       | TRUE      | 31822 |            | 2XMM J033255.5-092729 | -3.9    | 28.1  |
| 42075 | HR 1099                  | V711 Tau                | 0064 01568 1 | 6.1  | 0.9  | K2: Vnk     | RS CVn              | 31   | HIP     | TRUE       | TRUE      | 32605 |            | 2XMM J033647.2+003516 | -2.2    | 30.9  |
| 42078 | HR 1099                  | V711 Tau                | 0064 01568 1 | 6.1  | 0.9  | K2: Vnk     | RS CVn              | 31   | HIP     | TRUE       | TRUE      | 32605 |            | 2XMM J033647.2+003516 | -2.2    | 30.9  |
| 42082 | HR 1099                  | V711 Tau                | 0064 01568 1 | 6.1  | 0.9  | K2: Vnk     | RS CVn              | 31   | HIP     | TRUE       | TRUE      | 32605 |            | 2XMM J033647.2+003516 | -2.0    | 31.2  |
| 42073 | HR 1099                  | V711 Tau                | 0064 01568 1 | 6.1  | 0.9  | K2: Vnk     | RS CVn              | 31   | HIP     | TRUE       | TRUE      | 32605 |            | 2XMM J033647.2+003516 | -2.2    | 30.9  |
| 42842 | SDSS J033815.04+002926.0 |                         | 0064 01340 1 | 11.9 | 0.3  |             |                     | 710  | TYC     | FALSE      | TRUE      | 33211 |            | 2XMM J033815.0+002925 | -2.3    | 31.2  |
| 44374 | V471 Tau                 |                         | 1252 00212 1 | 9.6  | 0.8  | K2 V+DA     | SB                  | 44   | HIP     | TRUE       | TRUE      | 34580 |            | 2XMM J035024.9+171447 | -2.1    | 29.9  |
| 45610 | 2MASS J04072181-1210033  | TYC 5315-00102-1        | 5315 00102 1 | 11.7 | 0.5  |             | W UMa               | 396  | TYC     | FALSE      | TRUE      | 35718 |            | 2XMM J040721.7-121003 | -1.9    | 31.2  |
| 45611 | 2MASS J04072181-1210033  | TYC 5315-00102-1        | 5315 00102 1 | 11.7 | 0.5  |             | W UMa               | 396  | TYC     | FALSE      | TRUE      | 35718 |            | 2XMM J040721.7-121003 | -2.1    | 31.0  |
| 46637 | V410 Tau                 | HD 283518               | 1827 00008 1 | 11.1 | 1.4  | K4 IV       | T Tau               | 98   | HIP     | TRUE       | TRUE      | 36574 |            | 2XMM J041831.0+282716 | -1.6    | 30.6  |
| 46636 | V410 Tau                 | HD 283518               | 1827 00008 1 | 11.1 | 1.4  | K4 IV       | T Tau               | 98   | HIP     | TRUE       | FALSE     | 36574 |            | 2XMM J041831.0+282716 | -1.8    | 30.4  |
| 47912 | HD 283572                | V987 Tau                | 1828 00481 1 | 9.2  | 0.7  | G5 IV       | Orion-type variable | 128  | HIP     | TRUE       | TRUE      | 37582 |            | 2XMM J042158.8+281806 | -2.2    | 31.0  |
| 47918 | T Tau                    | HD 284419               | 1272 00470 1 | 10.1 | 1.1  | G5 V.e...   | T Tau               | 182  | HIP     | TRUE       | TRUE      | 37588 | 37584      | 2XMM J042159.4+193206 | -2.1    | 31.0  |
| 48185 | VB 50                    | HD 27836                | 0680 00146 1 | 7.7  | 0.6  | G1 V        |                     | 44   | HIP     | TRUE       | TRUE      | 37825 |            | 2XMM J042412.4+144529 | -2.9    | 29.9  |
| 48184 | VB 50                    | HD 27836                | 0680 00146 1 | 7.7  | 0.6  | G1 V        |                     | 44   | HIP     | TRUE       | TRUE      | 37825 |            | 2XMM J042412.4+144529 | -3.0    | 29.7  |
| 48976 | 78 Tau                   | HD 28319                | 1265 01172 1 | 3.4  | 0.2  | A7 III      | del Sct             | 46   | HIP     | FALSE      | TRUE      | 38388 |            | 2XMM J042839.7+155217 | -6.0    | 28.6  |
| 49620 | HD 285845                | V1073 Tau               | 1269 00469 1 | 10.5 | 0.7  | G6          | SB                  | 90   | F03     | TRUE       | TRUE      | 38879 |            | 2XMM J043125.1+181616 | -2.0    | 30.3  |
| 49707 | HD 28634                 | VB 285                  | 1269 01027 1 | 9.7  | 1.0  | K2          | SB                  | 44   | HIP     | TRUE       | TRUE      | 38940 |            | 2XMM J043137.0+174235 | -3.0    | 29.0  |
| 50256 | V807 Tau                 |                         | 1829 00214 1 | 11.4 | 0.9  | K5          | Orion-type variable | 140  | G07     | FALSE      | TRUE      | 39281 |            | 2XMM J043306.6+240954 | -2.3    | 30.1  |
| 51649 | HD 283810                |                         | 1834 00179 1 | 10.8 | 1.0  | K5 V        |                     | 60   | F07     | FALSE      | FALSE     | 40393 |            | 2XMM J044009.2+253533 | -2.0    | 29.9  |
| 53325 | HD 31305                 |                         | 2387 00171 1 | 7.6  | 0.1  | A0          |                     | 135  | N2K     | FALSE      | TRUE      | 41960 |            | 2XMM J045548.2+302016 | -3.5    | 30.3  |
| 53358 | SU Aur                   | HD 282624               | 2387 00977 1 | 9.6  | 0.9  | G2 III      | Orion-type variable | 146  | HIP     | TRUE       | TRUE      | 41991 |            | 2XMM J045559.3+303401 | -2.3    | 30.8  |
| 54373 | HD 268974                | ASAS J050527-6743.2     | 9161 01103 1 | 11.5 | 0.8  | K2          | EB                  | 917  | N2K     | FALSE      | TRUE      | 42946 |            | 2XMM J050526.8-674315 | -2.0    | 31.9  |
| 61209 | AB Dor                   | HD 36705                | 8887 01611 1 | 7.1  | 0.8  | K0 V        |                     | 15   | HIP     | TRUE       | TRUE      | 47464 |            | 2XMM J052844.7-652654 | -1.9    | 30.2  |
| 61210 | AB Dor                   | HD 36705                | 8887 01611 1 | 7.1  | 0.8  | K0 V        |                     | 15   | HIP     | TRUE       | TRUE      | 47464 |            | 2XMM J052844.7-652654 | -2.1    | 30.1  |
| 61212 | AB Dor                   | HD 36705                | 8887 01611 1 | 7.1  | 0.8  | K0 V        |                     | 15   | HIP     | TRUE       | TRUE      | 47464 |            | 2XMM J052844.7-652654 | -2.0    | 30.1  |
| 61217 | AB Dor                   | HD 36705                | 8887 01611 1 | 7.1  | 0.8  | K0 V        |                     | 15   | HIP     | TRUE       | TRUE      | 47464 |            | 2XMM J052844.7-652654 | -1.9    | 30.3  |
| 61223 | AB Dor                   | HD 36705                | 8887 01611 1 | 7.1  | 0.8  | K0 V        |                     | 15   | HIP     | TRUE       | TRUE      | 47464 |            | 2XMM J052844.7-652654 | -1.9    | 30.3  |
| 61222 | AB Dor                   | HD 36705                | 8887 01611 1 | 7.1  | 0.8  | K0 V        |                     | 15   | HIP     | TRUE       | TRUE      | 47464 |            | 2XMM J052844.7-652654 | -2.0    | 30.2  |
| 61224 | AB Dor                   | HD 36705                | 8887 01611 1 | 7.1  | 0.8  | K0 V        |                     | 15   | HIP     | TRUE       | TRUE      | 47464 |            | 2XMM J052844.7-652654 | -2.1    | 30.0  |
| 61213 | AB Dor                   | HD 36705                | 8887 01611 1 | 7.1  | 0.8  | K0 V        |                     | 15   | HIP     | TRUE       | TRUE      | 47464 |            | 2XMM J052844.7-652654 | -2.0    | 30.1  |
| 61219 | AB Dor                   | HD 36705                | 8887 01611 1 | 7.1  | 0.8  | K0 V        |                     | 15   | HIP     | TRUE       | TRUE      | 47464 |            | 2XMM J052844.7-652654 | -2.0    | 30.1  |
| 61221 | AB Dor                   | HD 36705                | 8887 01611 1 | 7.1  | 0.8  | K0 V        |                     | 15   | HIP     | TRUE       | FALSE     | 47464 |            | 2XMM J052844.7-652654 | -2.1    | 30.0  |
| 61220 | AB Dor                   | HD 36705                | 8887 01611 1 | 7.1  | 0.8  | K0 V        |                     | 15   | HIP     | TRUE       | FALSE     | 47464 |            | 2XMM J052844.7-652654 | -1.8    | 30.3  |
| 64214 | 2MASS J05350341-0505402  | GS C 04774-00868        | 4774 00868 1 | 10.6 | 0.3  |             |                     | 450  | T02     | FALSE      | FALSE     | 49678 |            | 2XMM J053503.4-050540 | -3.1    | 30.6  |
| 65197 | HD 37040                 |                         | 4774 00937 1 | 6.4  | -0.1 | B2.5 IV     |                     | 361  | HIP     | TRUE       | TRUE      | 50242 |            | 2XMM J053531.0-042151 | -4.0    | 31.1  |
| 71057 | chi01 Ori                | HD 39587                | 1320 02118 1 | 4.5  | 0.5  | G0 VCH-0.3  | SB PMS              | 9    | HIP     | TRUE       | FALSE     | 54947 |            | 2XMM J055422.8+201634 | -3.8    | 28.9  |
| 75409 | SV Cam                   | HD 44982                | 4538 00458 1 | 9.5  | 0.6  | G0V+K6V     | RS CVn, EB          | 88   | HIP     | TRUE       | TRUE      | 58326 |            | 2XMM J064119.1+821602 | -2.1    | 30.5  |
| 75410 | SV Cam                   | HD 44982                | 4538 00458 1 | 9.5  | 0.6  | G0V+K6V     | RS CVn, EB          | 88   | HIP     | TRUE       | TRUE      | 58326 |            | 2XMM J064119.1+821602 | -2.0    | 30.6  |
| 79319 | HD 51141                 |                         | 4622 00897 1 | 8.2  | 0.4  | F8          |                     | 79   | HIP     | FALSE      | TRUE      | 61056 |            | 2XMM J072524.9+854418 | -4.8    | 28.3  |
| 80086 | HD 59581                 |                         | 4124 00980 1 | 8.5  | 0.4  | F6          | active binary       | 103  | F95     | FALSE      | TRUE      | 61727 |            | 2XMM J073509.1+654024 | -3.2    | 30.0  |
| 81491 | YZ CMi                   | GJ 285                  | 0183 02190 1 | 11.5 | 1.5  | M4.5 Ve     | flare star          | 6    | HIP     | TRUE       | TRUE      | 62784 |            | 2XMM J074440.1+033308 | -1.0    | 28.5  |
| 89993 | 2MASS J08322856+5245330  |                         | 3797 01900 1 | 11.6 | 1.0  |             |                     | 18   | N2K     | FALSE      | TRUE      | 67988 |            | 2XMM J083228.6+524533 | -3.4    | 27.1  |
| 91247 | pi.01 UMa                | HD 72905                | 4133 01971 1 | 5.8  | 0.6  | G1.5 Vb     | BY Dra              | 14   | HIP     | TRUE       | FALSE     | 69047 |            | 2XMM J083911.7+650115 | -3.6    | 29.0  |
| 91420 | HD 73709                 |                         | 1395 02006 1 | 7.6  | 0.2  | F2 III      | SB1                 | 180  | R99     | FALSE      | TRUE      | 69219 |            | 2XMM J084020.7+194111 | -5.0    | 29.0  |

| DETID  | Star_Name               | Alt_Name                | Tycld        | Vmag | B-V | Star_SpType       | Star_Type           | Dist | DistRef | OBS_TARGET | CoolVflag | SRCID  | SrclidOther | IAUNAME               | logFx | Fv | logLx |
|--------|-------------------------|-------------------------|--------------|------|-----|-------------------|---------------------|------|---------|------------|-----------|--------|-------------|-----------------------|-------|----|-------|
| 93362  | CD-45 4602              |                         | 8152 00417 1 | 9.6  | 0.7 | G5                |                     | 72   | HIP     | FALSE      | TRUE      | 70721  |             | 2XMM J085002.4-454140 | -3.8  |    | 28.7  |
| 93359  | CD-45 4602              |                         | 8152 00417 1 | 9.6  | 0.7 | G5                |                     | 72   | HIP     | FALSE      | TRUE      | 70721  |             | 2XMM J085002.4-454140 | -3.5  |    | 29.0  |
| 95682  | XY UMa                  | HD 237786               | 3805 00027 1 | 9.7  | 0.8 | G3V + K4-5V       | RS CVn, EB          | 66   | HIP     | TRUE       | TRUE      | 72877  |             | 2XMM J090955.9+542917 | -2.1  |    | 30.3  |
| 98763  | LQ Hya                  | GJ 355                  | 5464 00875 1 | 8.0  | 0.9 | K0 V              | BY Dra              | 19   | HIP     | TRUE       | TRUE      | 75502  |             | 2XMM J093225.5-111104 | -2.1  |    | 29.8  |
| 98764  | LQ Hya                  | GJ 355                  | 5464 00875 1 | 8.0  | 0.9 | K0 V              | BY Dra              | 19   | HIP     | TRUE       | TRUE      | 75502  |             | 2XMM J093225.5-111104 | -2.1  |    | 29.9  |
| 99591  | HD 83698                | CCDM J09414+3857AB      | 2992 01245 1 | 7.3  | 0.7 | G5                | double star system  | 51   | HIP     | FALSE      | TRUE      | 76251  |             | 2XMM J094121.9+385659 | -4.9  |    | 28.2  |
| 101535 | 2MASS J09553615+6954487 |                         | 4383 00523 1 | 11.5 | 0.9 |                   |                     | 24   | N2K     | FALSE      | TRUE      | 77959  |             | 2XMM J095536.2+695448 | -2.5  |    | 28.2  |
| 108025 | AD Leo                  | GJ 388                  | 1423 00174 1 | 9.8  | 1.5 | M3.5 Ve           | flare star          | 5    | GCT     | TRUE       | TRUE      | 82640  |             | 2XMM J101936.1+195212 | -1.4  |    | 28.7  |
| 118876 | NU UMa                  | HD 237944               | 3829 00322 1 | 9.5  | 0.7 | G5                | EB                  | 106  | HIP     | FALSE      | FALSE     | 89750  |             | 2XMM J105300.9+574208 | -3.4  |    | 29.4  |
| 120401 | CR Cha                  |                         | 9414 00186 1 | 11.9 | 1.3 | K4 Ve             | Orion-type variable | 168  | HIP     | TRUE       | TRUE      | 90546  |             | 2XMM J105906.9-770140 | -2.0  |    | 30.3  |
| 121057 | HD 95735                | GI 411                  | 2521 02279 1 | 7.8  | 1.4 | M2 V              | flare star          | 3    | HIP     | FALSE      | TRUE      | 91087  | 91088       | 2XMM J110319.9+355750 | -4.1  |    | 26.2  |
| 123749 | GSC 09414-00787         | 2MASS J11061540-7721567 | 9414 00787 1 | 11.4 | 1.6 | G5 Ve             | PMS                 | 160  | S04     | TRUE       | TRUE      | 92587  |             | 2XMM J110615.5-772156 | -1.7  |    | 30.7  |
| 130963 | HD 104021               |                         | 8631 00350 1 | 7.5  | 0.2 | A7 V              |                     | 112  | HIP     | FALSE      | TRUE      | 99128  |             | 2XMM J115839.0-524607 | -3.0  |    | 30.7  |
| 142357 | HD 108984               |                         | 1447 00665 1 | 8.1  | 0.8 | K0 V              |                     | 26   | HIP     | FALSE      | TRUE      | 107354 |             | 2XMM J123118.3+201303 | -4.0  |    | 28.1  |
| 148010 | IM Vir                  | HD 111487               | 4955 00912 1 | 9.8  | 0.6 | G7+K7             | Algol               | 90   | M09     | FALSE      | TRUE      | 112107 |             | 2XMM J124938.6-060444 | -2.2  |    | 30.4  |
| 148011 | IM Vir                  | HD 111487               | 4955 00912 1 | 9.8  | 0.6 | G7+K7             | Algol               | 90   | M09     | FALSE      | TRUE      | 112107 |             | 2XMM J124938.6-060444 | -2.2  |    | 30.4  |
| 156921 | 2MASS J13141103-1620235 |                         | 6113 00581 1 | 11.9 | 0.5 |                   |                     | 516  | TYC     | FALSE      | TRUE      | 119315 |             | 2XMM J131410.9-162023 | -2.8  |    | 30.4  |
| 160700 | FK Com                  | HD 117555               | 1997 00553 1 | 8.4  | 0.9 | G4 III            | FK Com              | 168  | HIP     | TRUE       | TRUE      | 122713 |             | 2XMM J133046.8+241357 | -2.4  |    | 31.3  |
| 160701 | FK Com                  | HD 117555               | 1997 00553 1 | 8.4  | 0.9 | G4 III            | FK Com              | 168  | HIP     | TRUE       | TRUE      | 122713 |             | 2XMM J133046.8+241357 | -2.0  |    | 31.7  |
| 161095 | DG CVn                  | GJ 3789                 | 2003 00139 1 | 12.3 | 0.7 | M4 Ve             | BY Dra              | 8    | R95     | TRUE       | TRUE      | 123034 |             | 2XMM J133146.4+291635 | -1.3  |    | 28.2  |
| 163132 | 2MASS J13362690-3426365 |                         | 7273 01114 1 | 11.6 | 0.3 | K2                |                     | 100  | N2K     | FALSE      | TRUE      | 124412 |             | 2XMM J133626.8-342635 | -2.8  |    | 29.2  |
| 165709 | tau Boo                 | HD 120136               | 1460 00132 1 | 4.6  | 0.4 | F7 V              |                     | 16   | HIP     | TRUE       | FALSE     | 126786 |             | 2XMM J134715.6+172726 | -4.3  |    | 28.9  |
| 169401 | HD 122473               |                         | 5557 00199 1 | 8.7  | 1.0 | K0                |                     | 80   | N2K     | FALSE      | TRUE      | 130063 |             | 2XMM J140219.6-110459 | -4.1  |    | 28.8  |
| 170306 | GSC 03852-01069         | TYC 3852-1069-1         | 3852 01069 1 | 12.5 | 0.2 |                   |                     | 1463 | TYC     | FALSE      | TRUE      | 130617 |             | 2XMM J140421.6+541921 | -2.6  |    | 31.4  |
| 174625 | HD 127244               |                         | 3042 00305 1 | 9.2  | 0.6 | K0                |                     | 56   | N2K     | FALSE      | TRUE      | 133968 |             | 2XMM J142901.2+423050 | -3.8  |    | 28.7  |
| 175724 | EK Dra                  | HD 129333               | 4176 00540 1 | 7.7  | 0.6 | G1.5 V            | BY Dra              | 34   | HIP     | TRUE       | TRUE      | 134803 |             | 2XMM J143900.1+641729 | -2.5  |    | 30.1  |
| 177789 | xi Boo A                | HD 131156A              | 1481 00722 1 | 4.8  | 0.7 | G8 V              | flare star          | 7    | HIP     | TRUE       | TRUE      | 136487 |             | 2XMM J145123.3+190602 | -3.4  |    | 28.9  |
| 179597 | 44 Boo                  | HD 133640               | 3484 01580 1 | 5.3  | 0.5 | G0Vnv             | W UMa               | 13   | HIP     | TRUE       | FALSE     | 138085 |             | 2XMM J150347.4+473915 | -2.9  |    | 29.8  |
| 182638 | UZ Lib                  |                         | 5595 00180 1 | 9.4  | 1.0 | K0 III            | RS CVn              | 161  | HIP     | TRUE       | TRUE      | 140595 |             | 2XMM J153223.2-083200 | -1.9  |    | 31.4  |
| 187347 | sigma*2 CrB             | HD 146361               | 2583 01846 1 | 5.7  | 0.5 | F6 V+G0 V         | RS CVn              | 21   | HIP     | TRUE       | TRUE      | 144304 |             | 2XMM J161440.7+335129 | -2.3  |    | 30.7  |
| 193025 | CD-53 6825              |                         | 8713 02226 1 | 10.0 | 1.3 |                   |                     | 89   | N2K     | FALSE      | TRUE      | 148793 |             | 2XMM J164005.1-534530 | -2.9  |    | 29.6  |
| 194097 | alf TrA                 | HD 150798               | 9275 03641 1 | 2.2  | 1.5 | K2 II-III         |                     | 120  | HIP     | TRUE       | TRUE      | 149691 |             | 2XMM J164840.1-690139 | -5.6  |    | 30.2  |
| 194425 | TYC 9275-01654-1        |                         | 9275 01654 1 | 11.8 | 0.9 |                   |                     | 25   | N2K     | FALSE      | TRUE      | 149908 |             | 2XMM J165050.9-685914 | -2.1  |    | 28.6  |
| 204777 | BN Sgr                  | HD 161507               | 6840 00009 1 | 9.5  | 0.6 | F3 V              | Algol               | 400  | B04     | FALSE      | FALSE     | 157091 |             | 2XMM J174705.3-280859 | -3.1  |    | 30.8  |
| 210451 | 70 Oph                  | V2391 Oph               | 0434 05213 1 | 4.3  | 0.8 | K0 V + K5 V       | SB                  | 5    | HIP     | TRUE       | TRUE      | 162187 |             | 2XMM J180527.3+022955 | -4.1  |    | 28.2  |
| 212517 | HD 166191               |                         | 6843 01557 1 | 8.5  | 0.5 | F4 V              |                     | 119  | HIP     | FALSE      | TRUE      | 163742 |             | 2XMM J181030.3-233400 | -4.0  |    | 29.4  |
| 217384 | 2MASS J18403031+0513166 |                         | 0455 00921 1 | 12.0 | 1.5 |                   |                     | 76   | N2K     | FALSE      | TRUE      | 167716 |             | 2XMM J184030.1+051316 | -2.4  |    | 29.2  |
| 219667 | V709 CrA                |                         | 7421 01890 1 | 11.4 | 1.7 | K1 IV             | Orion-type variable | 130  | M81     | FALSE      | TRUE      | 169216 |             | 2XMM J190134.8-370056 | -1.1  |    | 31.2  |
| 224075 | TYC 1082-02107-1        |                         | 1082 02107 1 | 11.7 | 1.1 |                   |                     | 23   | N2K     | FALSE      | TRUE      | 172736 |             | 2XMM J201900.1+113507 | -2.6  |    | 28.0  |
| 226652 | VW Cep                  | HD 197433               | 4585 03284 1 | 7.7  | 0.8 | K0Vv              | W UMa               | 28   | HIP     | TRUE       | TRUE      | 174581 |             | 2XMM J203721.6+753603 | -2.6  |    | 29.8  |
| 226653 | VW Cep                  | HD 197433               | 4585 03284 1 | 7.7  | 0.8 | K0Vv              | W UMa               | 28   | HIP     | TRUE       | FALSE     | 174581 |             | 2XMM J203721.6+753603 | -2.6  |    | 29.8  |
| 226922 | AT Mic                  | HD 196982               | 7460 00137 1 | 11.5 | 1.1 | M4.5 Ve + M4.5 Ve | flare star          | 11   | HIP     | TRUE       | TRUE      | 174842 |             | 2XMM J204151.1-322607 | -0.6  |    | 29.5  |
| 227252 | AU Mic                  | HD 197481               | 7457 00641 1 | 9.1  | 1.5 | M0 Ve             | flare star          | 10   | HIP     | TRUE       | TRUE      | 175166 |             | 2XMM J204509.4-312028 | -1.5  |    | 29.4  |
| 229724 | 61 Cyg A                | HD 201091               | 3168 02800 1 | 5.5  | 1.2 | K5 V              | BY Dra              | 3    | HIP     | TRUE       | TRUE      | 177371 | 177369      | 2XMM J210655.3+384511 | -4.1  |    | 27.4  |
| 229734 | 61 Cyg B                | HD 201092               | 3168 02798 1 | 6.2  | 1.3 | K7 V              | flare star          | 3    | HIP     | TRUE       | TRUE      | 177375 | 177373      | 2XMM J210656.6+384444 | -4.4  |    | 26.8  |
| 229736 | 61 Cyg B                | HD 201092               | 3168 02798 1 | 6.2  | 1.3 | K7 V              | flare star          | 3    | HIP     | TRUE       | TRUE      | 177375 | 177373      | 2XMM J210656.6+384444 | -3.4  |    | 27.7  |
| 231002 | SAO 10050               | BD+69 1172              | 4465 00481 1 | 9.1  | 0.5 | F8                |                     | 73   | N2K     | FALSE      | TRUE      | 178313 |             | 2XMM J212707.5+702212 | -3.6  |    | 29.1  |
| 239075 | EV Lac                  | GJ 873A                 | 3226 02288 1 | 10.6 | 1.3 | M4.5 Ve           | flare star          | 5    | HIP     | TRUE       | TRUE      | 185001 |             | 2XMM J224649.6+442001 | -1.1  |    | 28.7  |
| 241508 | HK Aqr                  | GJ 890                  | 6395 00658 1 | 11.3 | 2.2 | M0 Ve             | BY Dra              | 22   | HIP     | TRUE       | TRUE      | 187121 |             | 2XMM J230819.6-152435 | -1.8  |    | 29.0  |
| 242179 | 1RXS J231628.7+790531   |                         | 4609 00273 1 | 11.2 | 0.8 |                   |                     | 55   | N2K     | FALSE      | TRUE      | 187670 |             | 2XMM J231630.5+790535 | -1.1  |    | 30.6  |
| 242641 | V368 Cep                | HD 220140               | 4609 00535 1 | 7.7  | 0.9 | G9 V              | RS CVn              | 19   | HIP     | TRUE       | TRUE      | 188039 |             | 2XMM J231926.6+790011 | -2.2  |    | 29.9  |
| 243984 | EQ Peg                  | GJ 896A                 | 1723 00023 1 | 10.7 | 1.5 | M3.5 Ve + M4.5 Ve | flare star          | 6    | HIP     | TRUE       | TRUE      | 189152 |             | 2XMM J233152.3+195614 | -1.1  |    | 28.8  |
| 243985 | EQ Peg                  | GJ 896A                 | 1723 00023 1 | 10.7 | 1.5 | M3.5 Ve + M4.5 Ve | flare star          | 6    | HIP     | FALSE      | TRUE      | 189152 |             | 2XMM J233152.3+195614 | -1.1  |    | 28.8  |
| 244744 | Iam And                 | HD 222107               | 3638 02515 1 | 4.1  | 1.0 | G8 IV-III         | RS CVn              | 26   | HIP     | TRUE       | TRUE      | 189774 |             | 2XMM J233733.8+462728 | -3.1  |    | 30.7  |

| DETID | Star_Name                | OBS_ID     | TSfile                      | MJD_START   | MJD_STOP    | OnTime | PN_FILTER | M1_FILTER | M2_FILTER | OFFAX_MIN | VAR_INST_ID | SUM_FLAG2 | NrEvents |
|-------|--------------------------|------------|-----------------------------|-------------|-------------|--------|-----------|-----------|-----------|-----------|-------------|-----------|----------|
| 1916  | UY Scl                   | 28740101   | P0028740101PNS003SRCTSR8003 | 52228.05250 | 52228.38015 | 30842  | Thin1     | Thin1     | Thin1     | 3.5       | PN          | 0         | 1        |
| 2236  | HD 1165                  | 112620201  | P0112620201M2S002SRCTSR8002 | 52144.17874 | 52144.63461 | 20452  | Medium    | Medium    | Medium    | 3.7       | M2          | 0         | 1        |
| 15656 | HD 8191                  | 11450101   | P0011450101PNS003SRCTSR8002 | 52060.12473 | 52060.77854 | 43157  | Thin1     | Thin1     | Thin1     | 6.2       | PN          | 1         | 1        |
| 22001 | 47 Cas B                 | 111520101  | P0111520101M1S001SRCTSR8001 | 52163.08648 | 52163.56215 | 40920  | UNDEF     | Thick     | Thick     | 0.1       | M1          | 0         | 1        |
| 23485 | HD 14716                 | 202130101  | P0202130101PNS003SRCTSR8001 | 53269.16483 | 53269.61513 | 25353  | Medium    | Medium    | Medium    | 0.7       | PN          | 1         | 1        |
| 30805 | CC Eri                   | 148790101  | P0148790101M1U002SRCTSR8001 | 52859.39000 | 52859.81480 | 32031  | Thick     | Thick     | Thick     | 0.1       | M1          | 2         | 2        |
| 32470 | CD-53 544                | 2027210101 | P0207210101M1S001SRCTSR8001 | 53044.89075 | 53045.33940 | 38076  | UNDEF     | Thin1     | Thin1     | 0.1       | M1          | 1         | 3        |
| 33241 | RZ Cas                   | 149040201  | P0149040201M2S002SRCTSR8001 | 52873.25118 | 52874.56421 | 64162  | Thick     | Thick     | Thick     | 0.2       | M2          | -3        | 6        |
| 37553 | kap01 Cet                | 111410101  | P0111410101M1S001SRCTSR8001 | 52314.68024 | 52315.13760 | 35336  | UNDEF     | Thick     | Medium    | 0.1       | M1          | 0         | 1        |
| 40682 | eps Eri                  | 112880501  | P0112880501PNS003SRCTSR8001 | 52658.50505 | 52658.63869 | 13111  | Thick     | Thick     | Thick     | 0.2       | PN          | -3        | 1        |
| 42075 | HR 1099                  | 134540101  | P0134540101PNS011SRCTSR8001 | 51962.60031 | 51962.71604 | 23626  | Medium    | Thick     | Thick     | 0.1       | PN          | -3        | 1        |
| 42078 | HR 1099                  | 129350201  | P0129350201PNS014SRCTSR8001 | 51784.29906 | 51784.36804 | 6643   | Thin1     | Thin1     | Thin1     | 0.2       | PN          | -3        | 1        |
| 42082 | HR 1099                  | 117890901  | P0117890901M2S004SRCTSR8001 | 51592.59370 | 51593.15670 | 36575  | Medium    | Medium    | Medium    | 6.1       | M2          | -3        | 1        |
| 42073 | HR 1099                  | 134540401  | P0134540401M2S007SRCTSR8001 | 52139.30963 | 52139.44484 | 11627  | UNDEF     | Thick     | Medium    | 0.2       | M2          | -3        | 1        |
| 42842 | S055 J033815.04+002926.0 | 36540101   | P0036540101M1S001SRCTSR8001 | 52327.36916 | 52327.60064 | 21752  | Thin1     | Thin1     | Thin1     | 8.5       | M1          | 0         | 1        |
| 44374 | V471 Tau                 | 203260101  | P0203260101M2S002SRCTSR8001 | 53218.28623 | 53218.98852 | 46825  | UNDEF     | Medium    | Medium    | 0.3       | M2          | -3        | 1        |
| 45610 | 2MASS J04072181-1210033  | 2022210301 | P0202210301M1S001SRCTSR8002 | 53403.75801 | 53404.68463 | 67684  | Thin1     | Thin1     | Thin1     | 6.2       | M1          | 0         | 2        |
| 45611 | 2MASS J04072181-1210033  | 2022210401 | P0202210401PNS003SRCTSR8002 | 53405.75245 | 53406.73926 | 73092  | Thin1     | Thin1     | Thin1     | 6.2       | PN          | 0         | 3        |
| 46637 | V410 Tau                 | 86360301   | P0086360301M1S005SRCTSR8001 | 51979.56233 | 51980.38198 | 62051  | Medium    | Medium    | Medium    | 0.1       | M1          | 0         | 1        |
| 46636 | V410 Tau                 | 86360401   | P0086360401PNU002SRCTSR8001 | 51980.43080 | 51980.90559 | 32282  | Medium    | Medium    | Medium    | 0.1       | PN          | 0         | 1        |
| 47912 | HD 283572                | 101440701  | P0101440701PNS003SRCTSR8001 | 51792.12343 | 51792.65828 | 32069  | Medium    | Medium    | Medium    | 0.1       | PN          | -3        | 1        |
| 47918 | T Tau                    | 301500101  | P0301500101PNS003SRCTSR8001 | 53597.59344 | 53598.53845 | 54964  | Medium    | Medium    | Medium    | 0.2       | PN          | -3        | 1        |
| 48185 | VB 50                    | 101440601  | P0101440601M2U002SRCTSR8001 | 51796.24407 | 51796.64878 | 42392  | Medium    | Medium    | Medium    | 0.0       | M2          | -3        | 1        |
| 48184 | VB 50                    | 101441501  | P0101441501PNU014SRCTSR8001 | 52338.74150 | 52339.28064 | 39504  | Medium    | Medium    | Medium    | 0.2       | PN          | 0         | 2        |
| 48976 | 78 Tau                   | 101440501  | P0101440501PNS003SRCTSR8003 | 51790.13105 | 51790.62539 | 40135  | Thick     | Thick     | Thick     | 5.6       | PN          | 1         | 2        |
| 49620 | HD 285845                | 109060301  | P0109060301M2S003SRCTSR8001 | 51796.79909 | 51797.43175 | 56851  | Medium    | Medium    | Medium    | 5.9       | M2          | -3        | 4        |
| 49707 | HD 28634                 | 94810301   | P0094810301M2S003SRCTSR8003 | 51619.00847 | 51619.32318 | 7735   | Thin1     | Thin1     | Thin1     | 8.9       | M2          | 0         | 1        |
| 50256 | V807 Tau                 | 203540401  | P0203540401PNS003SRCTSR8003 | 53422.06991 | 53422.43492 | 29592  | Medium    | Medium    | Medium    | 11.9      | PN          | 0         | 1        |
| 51649 | HD 283810                | 203540501  | P0203540501PNS003SRCTSR8001 | 53422.49178 | 53422.83988 | 19656  | Medium    | Medium    | Medium    | 8.8       | PN          | -3        | 1        |
| 53325 | HD 31305                 | 101440801  | P0101440801M2S002SRCTSR8003 | 52173.06547 | 52174.56494 | 126344 | UNDEF     | Thick     | Thick     | 13.9      | M2          | 0         | 1        |
| 53358 | SU Aur                   | 101440801  | P0101440801M2S002SRCTSR8001 | 52173.06547 | 52174.56494 | 126344 | UNDEF     | Thick     | Thick     | 0.1       | M2          | -3        | 3        |
| 54373 | HD 268974                | 201840101  | P0201840101PNS005SRCTSR8007 | 52986.86082 | 52987.55916 | 58838  | Medium    | Medium    | Medium    | 7.8       | PN          | -3        | 1        |
| 61209 | AB Dor                   | 134520301  | P0134520301M2S004SRCTSR8001 | 51929.64904 | 51930.22082 | 48802  | UNDEF     | Medium    | Medium    | 0.1       | M2          | -3        | 1        |
| 61210 | AB Dor                   | 134521301  | P0134521301M1S003SRCTSR8001 | 52195.47227 | 52195.92546 | 28362  | UNDEF     | Medium    | Medium    | 0.2       | M1          | -3        | 1        |
| 61212 | AB Dor                   | 134520701  | P0134520701M1S003SRCTSR8001 | 52051.70156 | 52052.26891 | 48891  | UNDEF     | Medium    | Medium    | 0.3       | M1          | -3        | 5        |
| 61217 | AB Dor                   | 134522101  | P0134522101M1S003SRCTSR8001 | 52638.45072 | 52639.01395 | 48630  | UNDEF     | Medium    | Medium    | 0.1       | M1          | 0         | 1        |
| 61223 | AB Dor                   | 134521701  | P0134521701M2S004SRCTSR8001 | 52593.23970 | 52593.46433 | 17420  | UNDEF     | Medium    | Medium    | 0.1       | M2          | 0         | 1        |
| 61222 | AB Dor                   | 133120201  | P0133120201M2S014SRCTSR8001 | 51890.82020 | 51890.86995 | 6189   | Thick     | Thick     | Thick     | 1.4       | M2          | -3        | 1        |
| 61224 | AB Dor                   | 123720301  | P0123720301M1S003SRCTSR8001 | 51844.63201 | 51845.28073 | 4316   | UNDEF     | Medium    | Medium    | 0.1       | M1          | 0         | 4        |
| 61213 | AB Dor                   | 134522301  | P0134522301M2U002SRCTSR8001 | 52728.84719 | 52728.89346 | 1508   | UNDEF     | Medium    | Medium    | 0.1       | M2          | -3        | 1        |
| 61219 | AB Dor                   | 134521601  | P0134521601M1S011SRCTSR8001 | 52443.68549 | 52443.88529 | 11440  | UNDEF     | Medium    | Medium    | 0.1       | M1          | -3        | 1        |
| 61221 | AB Dor                   | 160362701  | P0160362701M1S012SRCTSR8001 | 52936.14093 | 52936.34384 | 5080   | UNDEF     | Medium    | Medium    | 0.1       | M1          | -3        | 1        |
| 61220 | AB Dor                   | 134522001  | P0134522001M1S003SRCTSR8001 | 52611.20833 | 52611.42922 | 4264   | UNDEF     | Medium    | Medium    | 0.1       | M1          | 0         | 1        |
| 64214 | 2MASS J05350341-0505402  | 134531601  | P0134531601M1S002SRCTSR8028 | 52713.96348 | 52714.19369 | 20688  | Medium    | Medium    | Medium    | 5.1       | M1          | 0         | 1        |
| 65197 | HD 37040                 | 49560301   | P0049560301M1S001SRCTSR8007 | 52532.31613 | 52532.49569 | 21357  | Thick     | Thick     | Thick     | 13.3      | M1          | 6         | 1        |
| 71057 | chi01 Ori                | 111500101  | P0111500101M2S011SRCTSR8001 | 52006.37721 | 52006.73970 | 1300   | UNDEF     | UNDEF     | Thick     | 1.2       | M2          | 0         | 1        |
| 75409 | SV Cam                   | 29340101   | P0029340101PNU003SRCTSR8001 | 51996.09228 | 51996.40813 | 40899  | Medium    | Medium    | Medium    | 0.2       | PN          | -3        | 2        |
| 75410 | SV Cam                   | 29340201   | P0029340201M1S001SRCTSR8001 | 52917.57641 | 52918.22119 | 57817  | Medium    | Medium    | Medium    | 0.2       | M1          | -3        | 1        |
| 79319 | HD 51141                 | 22340201   | P0022340201PNU002SRCTSR8009 | 51984.26525 | 51984.83972 | 53866  | Thin1     | Thin1     | Thin1     | 6.9       | PN          | 0         | 1        |
| 80086 | HD 59581                 | 164560901  | P0164560901M1S001SRCTSR8003 | 53260.73227 | 53261.63068 | 69800  | Medium    | Medium    | Medium    | 13.7      | M1          | -3        | 1        |
| 81491 | YZ CMI                   | 111460101  | P0111460101M1S001SRCTSR8001 | 51826.27912 | 51826.58346 | 26078  | UNDEF     | Medium    | Medium    | 0.1       | M1          | 0         | 3        |
| 89993 | 2MASS J08322856+5245330  | 92800201   | P0092800201M2S003SRCTSR800F | 52392.73676 | 52393.89534 | 78185  | Medium    | Medium    | Medium    | 7.0       | M2          | 0         | 1        |
| 91247 | pi.01 UMa                | 111400101  | P0111400101M1S001SRCTSR8001 | 51851.91199 | 51852.49241 | 29385  | UNDEF     | Thick     | Thick     | 0.1       | M1          | 0         | 2        |
| 91420 | HD 73709                 | 101440401  | P0101440401M2S002SRCTSR801A | 51855.92653 | 51856.42420 | 45388  | Medium    | Thick     | Thick     | 9.4       | M2          | 1         | 1        |

| DETID  | Star_Name               | OBS_ID    | TSfile                      | MJD_START   | MJD_STOP    | OnTime | PN_FILTER | M1_FILTER | M2_FILTER | OFFAX_MIN | VAR_INST_ID | SUM_FLAG2 | NrEvents |
|--------|-------------------------|-----------|-----------------------------|-------------|-------------|--------|-----------|-----------|-----------|-----------|-------------|-----------|----------|
| 93362  | CD-45 4602              | 162360101 | P0162360101PNS003SRCTSR8003 | 52953.33794 | 52953.81035 | 29385  | Medium    | Medium    | Medium    | 6.8       | PN          | -3        | 1        |
| 93359  | CD-45 4602              | 112870301 | P0112870301PNS003SRCTSR8004 | 52024.11514 | 52024.38169 | 31137  | Medium    | Medium    | Medium    | 11.0      | PN          | -3        | 1        |
| 95682  | XY UMa                  | 200960101 | P0200960101PNS003SRCTSR8001 | 53457.98155 | 53458.95973 | 68570  | Medium    | Medium    | Medium    | 0.2       | PN          | -3        | 3        |
| 98763  | LQ Hya                  | 148880101 | P0148880101M2S002SRCTSR8001 | 52768.20318 | 52768.74228 | 33228  | UNDEF     | Thick     | Thick     | 0.1       | M2          | 0         | 1        |
| 98764  | LQ Hya                  | 148880301 | P0148880301M1S001SRCTSR8001 | 52965.35071 | 52965.53196 | 15568  | UNDEF     | Thick     | Thick     | 0.1       | M1          | 0         | 2        |
| 99591  | HD 83698                | 203270101 | P0203270101PNS003SRCTSR8002 | 53142.71522 | 53143.25961 | 48074  | Medium    | Medium    | Medium    | 4.2       | PN          | 0         | 1        |
| 101535 | 2MASS J09553615+6954487 | 206080101 | P0206080101M1S001SRCTSR8012 | 53116.91639 | 53118.10866 | 73369  | Medium    | Medium    | Medium    | 13.6      | M1          | 0         | 1        |
| 108025 | AD Leo                  | 111440101 | P0111440101M2S012SRCTSR8001 | 52043.87803 | 52044.28301 | 34356  | UNDEF     | Medium    | Thick     | 0.1       | M2          | -3        | 5        |
| 118876 | NU UMa                  | 147511601 | P0147511601M2S002SRCTSR8005 | 52605.97703 | 52607.41350 | 90082  | Medium    | Medium    | Medium    | 12.4      | M2          | 0         | 1        |
| 120401 | CR Cha                  | 67140201  | P0067140201PNS003SRCTSR8001 | 51964.24325 | 51964.65325 | 37952  | Medium    | Medium    | Medium    | 0.2       | PN          | -3        | 1        |
| 121057 | HD 95735                | 205370101 | P0205370101PNS003SRCTSR8001 | 53136.76301 | 53137.23616 | 40701  | Thin1     | Thin1     | Thin1     | 3.7       | PN          | -3        | 2        |
| 123749 | GSC 09414-00787         | 203810201 | P0203810201PNS003SRCTSR8001 | 53062.70013 | 53063.03388 | 29735  | Medium    | Medium    | Medium    | 10.3      | PN          | -3        | 1        |
| 130963 | HD 104021               | 301430101 | P0301430101PNS003SRCTSR8001 | 53736.81618 | 53737.24266 | 31541  | Thin1     | Thin1     | Thin1     | 7.6       | PN          | -3        | 1        |
| 142357 | HD 108984               | 301450201 | P0301450201M1S001SRCTSR8002 | 53560.53580 | 53560.82891 | 23764  | UNDEF     | Medium    | Medium    | 11.2      | M1          | 0         | 1        |
| 148010 | IM Vir                  | 203270301 | P0203270301PNU002SRCTSR8001 | 53201.23110 | 53201.82227 | 46475  | Medium    | Medium    | Medium    | 7.6       | PN          | -3        | 2        |
| 148011 | IM Vir                  | 60370201  | P0060370201PNS003SRCTSR8001 | 52101.66648 | 52102.10639 | 40379  | Thin1     | Thin1     | Thin1     | 7.5       | PN          | -3        | 2        |
| 156921 | 2MASS J13141103-1620235 | 301290101 | P0301290101M2S011SRCTSR8004 | 53741.42405 | 53742.07147 | 54449  | Thin1     | Thin1     | Thin1     | 3.9       | M2          | 1         | 1        |
| 160700 | FK Com                  | 100240201 | P0100240201PNS001SRCTSR8001 | 51930.73223 | 51931.15042 | 35785  | Medium    | Medium    | Medium    | 0.1       | PN          | -3        | 1        |
| 160701 | FK Com                  | 100240101 | P0100240101M1S002SRCTSR8001 | 51918.01492 | 51918.33263 | 29485  | Medium    | Medium    | Medium    | 0.1       | M1          | -3        | 1        |
| 161095 | DG Cvn                  | 301040101 | P0301040101PNS003SRCTSR8001 | 53723.71887 | 53724.06576 | 31923  | Medium    | Medium    | Medium    | 0.2       | PN          | -3        | 4        |
| 163132 | 2MASS J13362690-3426365 | 29740101  | P0029740101M2S002SRCTSR8002 | 52121.64149 | 52122.59435 | 63479  | UNDEF     | Medium    | Medium    | 10.4      | M2          | 0         | 1        |
| 165709 | tau Boo                 | 144570101 | P0144570101PNS003SRCTSR8001 | 52814.15711 | 52814.90241 | 55095  | Thick     | Thick     | Thick     | 0.1       | PN          | 0         | 1        |
| 169401 | HD 122473               | 109910101 | P0109910101PNS005SRCTSR8007 | 51920.44064 | 51920.96586 | 48984  | Thin1     | Thin1     | Thin1     | 10.4      | PN          | 0         | 1        |
| 170306 | GSC 03852-01069         | 212480201 | P0212480201PNS003SRCTSR8004 | 53378.58715 | 53378.94059 | 24498  | Thin1     | Thin1     | Thin1     | 6.4       | PN          | 0         | 1        |
| 174625 | HD 127244               | 310190101 | P0310190101M2S002SRCTSR8005 | 53540.31984 | 53540.86248 | 35150  | UNDEF     | Medium    | Medium    | 10.2      | M2          | 0         | 1        |
| 175724 | EK Dra                  | 111530101 | P0111530101PNS003SRCTSR8001 | 51908.61481 | 51909.19409 | 52023  | Thick     | Thick     | Thick     | 0.1       | PN          | -3        | 1        |
| 177789 | xi Boo A                | 56030101  | P0056030101M2S401SRCTSR8001 | 51928.47576 | 51929.15168 | 58838  | UNDEF     | Medium    | Medium    | 0.2       | M2          | 0         | 2        |
| 179597 | 44 Boo                  | 100650101 | P0100650101PNS003SRCTSR8001 | 52068.47728 | 52068.83395 | 17532  | Thick     | Thick     | Thick     | 0.1       | PN          | -3        | 3        |
| 182638 | UZ Lib                  | 100240801 | P0100240801PNS001SRCTSR8001 | 51940.84122 | 51941.12998 | 24924  | Medium    | Medium    | Medium    | 0.2       | PN          | -3        | 1        |
| 187347 | sigma*2 CrB             | 111470301 | P0111470301M2S002SRCTSR8001 | 52327.97913 | 52328.22736 | 7020   | UNDEF     | Thick     | Medium    | 0.2       | M2          | -3        | 1        |
| 193025 | CD-53 6825              | 105470401 | P0105470401M2S003SRCTSR8001 | 52145.36729 | 52145.60586 | 20459  | UNDEF     | Medium    | Medium    | 7.4       | M2          | 3         | 1        |
| 194097 | alf TrA                 | 21750501  | P0021750501PNS006SRCTSR8001 | 51971.90808 | 51972.19453 | 27684  | Thick     | Thick     | Thick     | 0.1       | PN          | 0         | 3        |
| 194425 | TVC 9275-01654-1        | 21750701  | P0021750701M1S004SRCTSR8003 | 51972.32522 | 51972.62208 | 28262  | Thick     | Thick     | Thick     | 11.0      | M1          | 1         | 1        |
| 204777 | BN Sgr                  | 112970201 | P0112970201PNS003SRCTSR8001 | 51810.99167 | 51811.15041 | 17389  | Medium    | Medium    | Medium    | 2.5       | PN          | 0         | 1        |
| 210451 | 70 Oph                  | 44741301  | P0044741301PNS002SRCTSR8001 | 52893.20361 | 52893.29083 | 9165   | Thick     | Thick     | Thick     | 0.0       | PN          | 1         | 1        |
| 212517 | HD 166191               | 201270101 | P0201270101M2S002SRCTSR8003 | 53280.31924 | 53281.12331 | 56033  | UNDEF     | Medium    | Medium    | 8.8       | M2          | -3        | 1        |
| 217384 | 2MASS J18403031+0513166 | 84020601  | P0084020601M2S003SRCTSR8002 | 53090.60855 | 53090.85707 | 21141  | UNDEF     | Thick     | Thick     | 13.3      | M2          | 0         | 1        |
| 219667 | V709 CrA                | 146390101 | P0146390101PNS005SRCTSR8002 | 52726.36858 | 52726.77279 | 21476  | Medium    | Medium    | Medium    | 8.6       | PN          | 1         | 1        |
| 224075 | TVC 1082-02107-1        | 112960501 | P0112960501PNS003SRCTSR8001 | 52570.07833 | 52570.24207 | 14360  | Medium    | Medium    | Medium    | 9.2       | PN          | 0         | 1        |
| 226652 | VW Cep                  | 100650301 | P0100650301PNS003SRCTSR8001 | 52577.26440 | 52577.38067 | 11611  | Thick     | Thick     | Thick     | 0.1       | PN          | 0         | 1        |
| 226653 | VW Cep                  | 100650201 | P0100650201M2S002SRCTSR8001 | 52549.38613 | 52549.57090 | 6916   | Thick     | Thick     | Thick     | 0.2       | M2          | 1         | 1        |
| 226922 | AT Mic                  | 111510101 | P0111510101M1S001SRCTSR8001 | 51833.01961 | 51833.31358 | 18432  | UNDEF     | Medium    | Medium    | 0.0       | M1          | 0         | 1        |
| 227252 | AU Mic                  | 111420101 | P0111420101M1S001SRCTSR8001 | 51830.64338 | 51831.28341 | 55179  | UNDEF     | Thick     | Medium    | 0.1       | M1          | 0         | 6        |
| 229724 | 61 Cyg A                | 41741001  | P0041741001PNS003SRCTSR8001 | 52965.04980 | 52965.12734 | 8175   | Thick     | Thick     | Thick     | 0.6       | PN          | 1         | 1        |
| 229734 | 61 Cyg B                | 41741101  | P0041741101PNU002SRCTSR8002 | 53126.65183 | 53126.79985 | 14245  | Thick     | Thick     | Thick     | 0.5       | PN          | 1         | 1        |
| 229736 | 61 Cyg B                | 143630101 | P0143630101M2S002SRCTSR8001 | 53311.98000 | 53312.14118 | 15973  | Thick     | Thick     | Thick     | 0.6       | M2          | 1         | 1        |
| 231002 | SAO 10050               | 300490501 | P0300490501M2S002SRCTSR8002 | 53588.21576 | 53588.72969 | 39469  | UNDEF     | Thick     | Thick     | 13.0      | M2          | 0         | 1        |
| 239075 | EV Lac                  | 111450101 | P0111450101M2S011SRCTSR8001 | 52063.32998 | 52063.70047 | 28449  | UNDEF     | Medium    | Medium    | 0.1       | M2          | 0         | 6        |
| 241508 | HK Aqr                  | 202360101 | P0202360101M1S001SRCTSR8001 | 53507.47727 | 53508.69059 | 74204  | UNDEF     | Medium    | Medium    | 0.1       | M1          | 0         | 4        |
| 242179 | 1RXS J231628.7+790531   | 203060101 | P0203060101M2S002SRCTSR8002 | 53000.80814 | 53001.15260 | 28714  | UNDEF     | Thick     | Thick     | 10.0      | M2          | -3        | 1        |
| 242641 | V368 Cep                | 203060101 | P0203060101M1S001SRCTSR8001 | 53000.80814 | 53001.15260 | 28721  | UNDEF     | Thick     | Thick     | 0.1       | M1          | 0         | 3        |
| 243984 | EQ Peg                  | 112880301 | P0112880301PNS003SRCTSR8001 | 51734.51407 | 51734.65770 | 14415  | Thick     | Thick     | Thick     | 0.7       | PN          | -3        | 1        |
| 243985 | EQ Peg                  | 147580301 | P0147580301PNS003SRCTSR8001 | 52635.88793 | 52636.04414 | 12464  | Thin1     | Thin1     | Thin1     | 11.4      | PN          | -3        | 1        |
| 244744 | lam And                 | 99320101  | P0099320101M2S401SRCTSR8001 | 51935.84789 | 51936.17139 | 28496  | UNDEF     | Thick     | Thick     | 0.1       | M2          | 0         | 1        |

| DETID | Star_Name                | Star_Notes               | Star_Ref                   | XMM_Ref                                         | DPsummaryLink                                                                                                                                                                           |
|-------|--------------------------|--------------------------|----------------------------|-------------------------------------------------|-----------------------------------------------------------------------------------------------------------------------------------------------------------------------------------------|
| 1916  | UY Scl                   |                          | Chen+ 2006                 | Stobbs+ 2006                                    | <a href="http://www.ledas.ac.uk/data/2XMM/0354_0028740101_002/C0028740101EPX000SRCSUM0003.HTM">http://www.ledas.ac.uk/data/2XMM/0354_0028740101_002/C0028740101EPX000SRCSUM0003.HTM</a> |
| 2236  | HD 1165                  |                          |                            |                                                 | <a href="http://www.ledas.ac.uk/data/2XMM/0312_0112620201_003/C0112620201EPX000SRCSUM0002.HTM">http://www.ledas.ac.uk/data/2XMM/0312_0112620201_003/C0112620201EPX000SRCSUM0002.HTM</a> |
| 15656 | HD 8191                  | period ~19 dy?           | Koen+ 2002                 |                                                 | <a href="http://www.ledas.ac.uk/data/2XMM/0270_0011450101_002/C0011450101EPX000SRCSUM0002.HTM">http://www.ledas.ac.uk/data/2XMM/0270_0011450101_002/C0011450101EPX000SRCSUM0002.HTM</a> |
| 22001 | 47 Cas B                 |                          |                            | Telleschi+ 2005; Nordon+ 2008                   | <a href="http://www.ledas.ac.uk/data/2XMM/0322_0111520101_003/C0111520101EPX000SRCSUM0001.HTM">http://www.ledas.ac.uk/data/2XMM/0322_0111520101_003/C0111520101EPX000SRCSUM0001.HTM</a> |
| 23485 | HD 14716                 |                          |                            |                                                 | <a href="http://www.ledas.ac.uk/data/2XMM/0876_0202130101_001/C0202130101EPX000SRCSUM0001.HTM">http://www.ledas.ac.uk/data/2XMM/0876_0202130101_001/C0202130101EPX000SRCSUM0001.HTM</a> |
| 30805 | CC Eri                   |                          |                            | Crespo-Chacon+ 2007; Nordon+ 2008; Pandey+ 2008 | <a href="http://www.ledas.ac.uk/data/2XMM/0671_0148790101_003/C0148790101EPX000SRCSUM0001.HTM">http://www.ledas.ac.uk/data/2XMM/0671_0148790101_003/C0148790101EPX000SRCSUM0001.HTM</a> |
| 32470 | CD-53 544                |                          |                            |                                                 | <a href="http://www.ledas.ac.uk/data/2XMM/0764_0207210101_002/C0207210101EPX000SRCSUM0001.HTM">http://www.ledas.ac.uk/data/2XMM/0764_0207210101_002/C0207210101EPX000SRCSUM0001.HTM</a> |
| 33241 | RZ Cas                   |                          |                            |                                                 | <a href="http://www.ledas.ac.uk/data/2XMM/0678_0149040201_002/C0149040201EPX000SRCSUM0001.HTM">http://www.ledas.ac.uk/data/2XMM/0678_0149040201_002/C0149040201EPX000SRCSUM0001.HTM</a> |
| 37553 | kap01 Cet                |                          |                            | Telleschi+ 2005                                 | <a href="http://www.ledas.ac.uk/data/2XMM/0398_0111410101_002/C0111410101EPX000SRCSUM0001.HTM">http://www.ledas.ac.uk/data/2XMM/0398_0111410101_002/C0111410101EPX000SRCSUM0001.HTM</a> |
| 40682 | eps Eri                  |                          |                            |                                                 | <a href="http://www.ledas.ac.uk/data/2XMM/0570_0112880501_002/C0112880501EPX000SRCSUM0001.HTM">http://www.ledas.ac.uk/data/2XMM/0570_0112880501_002/C0112880501EPX000SRCSUM0001.HTM</a> |
| 42075 | HR 1099                  |                          |                            | Audard+ 2001; Nordon+ 2008; Pandey+ 2012        | <a href="http://www.ledas.ac.uk/data/2XMM/0221_0134540101_002/C0134540101EPX000SRCSUM0001.HTM">http://www.ledas.ac.uk/data/2XMM/0221_0134540101_002/C0134540101EPX000SRCSUM0001.HTM</a> |
| 42078 | HR 1099                  |                          |                            | Audard+ 2001; Nordon+ 2008; Pandey+ 2012        | <a href="http://www.ledas.ac.uk/data/2XMM/0132_0129350201_004/C0129350201EPX000SRCSUM0001.HTM">http://www.ledas.ac.uk/data/2XMM/0132_0129350201_004/C0129350201EPX000SRCSUM0001.HTM</a> |
| 42082 | HR 1099                  |                          |                            | Audard+ 2001; Nordon+ 2008; Pandey+ 2012        | <a href="http://www.ledas.ac.uk/data/2XMM/0036_0117890901_001/C0117890901EPX000SRCSUM0001.HTM">http://www.ledas.ac.uk/data/2XMM/0036_0117890901_001/C0117890901EPX000SRCSUM0001.HTM</a> |
| 42073 | HR 1099                  |                          |                            | Audard+ 2001; Nordon+ 2008; Pandey+ 2012        | <a href="http://www.ledas.ac.uk/data/2XMM/0310_0134540401_002/C0134540401EPX000SRCSUM0001.HTM">http://www.ledas.ac.uk/data/2XMM/0310_0134540401_002/C0134540401EPX000SRCSUM0001.HTM</a> |
| 42842 | SDSS J033815.04+002926.0 |                          |                            |                                                 | <a href="http://www.ledas.ac.uk/data/2XMM/0404_0036540101_002/C0036540101EPX000SRCSUM0001.HTM">http://www.ledas.ac.uk/data/2XMM/0404_0036540101_002/C0036540101EPX000SRCSUM0001.HTM</a> |
| 44374 | V471 Tau                 |                          |                            | Pandey+ 2008                                    | <a href="http://www.ledas.ac.uk/data/2XMM/0851_0203260101_001/C0203260101EPX000SRCSUM0001.HTM">http://www.ledas.ac.uk/data/2XMM/0851_0203260101_001/C0203260101EPX000SRCSUM0001.HTM</a> |
| 45610 | 2MASS J04072181-1210033  |                          | Farrell+ 2009; West 2009   |                                                 | <a href="http://www.ledas.ac.uk/data/2XMM/0944_0202210301_001/C0202210301EPX000SRCSUM0002.HTM">http://www.ledas.ac.uk/data/2XMM/0944_0202210301_001/C0202210301EPX000SRCSUM0002.HTM</a> |
| 45611 | 2MASS J04072181-1210033  |                          | Farrell+ 2009; West 2009   |                                                 | <a href="http://www.ledas.ac.uk/data/2XMM/0945_0202210401_001/C0202210401EPX000SRCSUM0002.HTM">http://www.ledas.ac.uk/data/2XMM/0945_0202210401_001/C0202210401EPX000SRCSUM0002.HTM</a> |
| 46637 | V410 Tau                 |                          |                            | Audard+ 2007; Franciosini+ 2007a; Guedel+ 2007a | <a href="http://www.ledas.ac.uk/data/2XMM/0230_0086360301_002/C0086360301EPX000SRCSUM0001.HTM">http://www.ledas.ac.uk/data/2XMM/0230_0086360301_002/C0086360301EPX000SRCSUM0001.HTM</a> |
| 46636 | V410 Tau                 |                          |                            | Audard+ 2007; Franciosini+ 2007a; Guedel+ 2007a | <a href="http://www.ledas.ac.uk/data/2XMM/0230_0086360401_002/C0086360401EPX000SRCSUM0001.HTM">http://www.ledas.ac.uk/data/2XMM/0230_0086360401_002/C0086360401EPX000SRCSUM0001.HTM</a> |
| 47912 | HD 283572                |                          |                            | Guedel+ 2007a                                   | <a href="http://www.ledas.ac.uk/data/2XMM/0136_0101440701_005/C0101440701EPX000SRCSUM0001.HTM">http://www.ledas.ac.uk/data/2XMM/0136_0101440701_005/C0101440701EPX000SRCSUM0001.HTM</a> |
| 47918 | T Tau                    |                          |                            | Audard+ 2007; Guedel+ 2007a,b                   | <a href="http://www.ledas.ac.uk/data/2XMM/1041_0301500101_002/C0301500101EPX000SRCSUM0001.HTM">http://www.ledas.ac.uk/data/2XMM/1041_0301500101_002/C0301500101EPX000SRCSUM0001.HTM</a> |
| 48185 | VB 50                    | in Hyades open cluster   |                            | Pallavicini+ 2004                               | <a href="http://www.ledas.ac.uk/data/2XMM/0138_0101440601_004/C0101440601EPX000SRCSUM0001.HTM">http://www.ledas.ac.uk/data/2XMM/0138_0101440601_004/C0101440601EPX000SRCSUM0001.HTM</a> |
| 48184 | VB 50                    | in Hyades open cluster   |                            | Pallavicini+ 2004                               | <a href="http://www.ledas.ac.uk/data/2XMM/0410_0101441501_002/C0101441501EPX000SRCSUM0001.HTM">http://www.ledas.ac.uk/data/2XMM/0410_0101441501_002/C0101441501EPX000SRCSUM0001.HTM</a> |
| 48976 | 78 Tau                   | in Hyades open cluster   |                            | Pallavicini+ 2004                               | <a href="http://www.ledas.ac.uk/data/2XMM/0135_0101440501_005/C0101440501EPX000SRCSUM0003.HTM">http://www.ledas.ac.uk/data/2XMM/0135_0101440501_005/C0101440501EPX000SRCSUM0003.HTM</a> |
| 49620 | HD 285845                | foreground star to L1551 | Walter+ 1988; Favata+ 2003 | Favata+ 2003; Franciosini+ 2007a                | <a href="http://www.ledas.ac.uk/data/2XMM/0138_0109060301_004/C0109060301EPX000SRCSUM0001.HTM">http://www.ledas.ac.uk/data/2XMM/0138_0109060301_004/C0109060301EPX000SRCSUM0001.HTM</a> |
| 49707 | HD 28634                 | in Hyades open cluster   |                            |                                                 | <a href="http://www.ledas.ac.uk/data/2XMM/0049_0094810301_002/C0094810301EPX000SRCSUM0003.HTM">http://www.ledas.ac.uk/data/2XMM/0049_0094810301_002/C0094810301EPX000SRCSUM0003.HTM</a> |
| 50256 | V807 Tau                 |                          |                            | Guedel+ 2007a                                   | <a href="http://www.ledas.ac.uk/data/2XMM/0953_0203540401_001/C0203540401EPX000SRCSUM0003.HTM">http://www.ledas.ac.uk/data/2XMM/0953_0203540401_001/C0203540401EPX000SRCSUM0003.HTM</a> |
| 51649 | HD 283810                | foreground star to TMC   |                            | Franciosini+ 2007a                              | <a href="http://www.ledas.ac.uk/data/2XMM/0953_0203540501_001/C0203540501EPX000SRCSUM0001.HTM">http://www.ledas.ac.uk/data/2XMM/0953_0203540501_001/C0203540501EPX000SRCSUM0001.HTM</a> |
| 53325 | HD 31305                 |                          |                            | Arzner+ 2007; Franciosini+ 2007b                | <a href="http://www.ledas.ac.uk/data/2XMM/0327_0101440801_003/C0101440801EPX000SRCSUM0003.HTM">http://www.ledas.ac.uk/data/2XMM/0327_0101440801_003/C0101440801EPX000SRCSUM0003.HTM</a> |
| 53358 | SU Aur                   |                          |                            | Robrade+ 2006; Franciosini+ 2007b               | <a href="http://www.ledas.ac.uk/data/2XMM/0327_0101440801_003/C0101440801EPX000SRCSUM0001.HTM">http://www.ledas.ac.uk/data/2XMM/0327_0101440801_003/C0101440801EPX000SRCSUM0001.HTM</a> |
| 54373 | HD 268974                | foreground star to LMC   | Pojmanski+ 1998; West 2009 |                                                 | <a href="http://www.ledas.ac.uk/data/2XMM/0735_0201840101_002/C0201840101EPX000SRCSUM0007.HTM">http://www.ledas.ac.uk/data/2XMM/0735_0201840101_002/C0201840101EPX000SRCSUM0007.HTM</a> |
| 61209 | AB Dor                   |                          |                            | Guedel+ 2001; Matranga+ 2005                    | <a href="http://www.ledas.ac.uk/data/2XMM/0205_0134520301_002/C0134520301EPX000SRCSUM0001.HTM">http://www.ledas.ac.uk/data/2XMM/0205_0134520301_002/C0134520301EPX000SRCSUM0001.HTM</a> |
| 61210 | AB Dor                   |                          |                            | Guedel+ 2001; Matranga+ 2005                    | <a href="http://www.ledas.ac.uk/data/2XMM/0338_0134521301_002/C0134521301EPX000SRCSUM0001.HTM">http://www.ledas.ac.uk/data/2XMM/0338_0134521301_002/C0134521301EPX000SRCSUM0001.HTM</a> |
| 61212 | AB Dor                   |                          |                            | Guedel+ 2001; Matranga+ 2005                    | <a href="http://www.ledas.ac.uk/data/2XMM/0266_0134520701_002/C0134520701EPX000SRCSUM0001.HTM">http://www.ledas.ac.uk/data/2XMM/0266_0134520701_002/C0134520701EPX000SRCSUM0001.HTM</a> |
| 61217 | AB Dor                   |                          |                            | Guedel+ 2001; Matranga+ 2005                    | <a href="http://www.ledas.ac.uk/data/2XMM/0560_0134522101_002/C0134522101EPX000SRCSUM0001.HTM">http://www.ledas.ac.uk/data/2XMM/0560_0134522101_002/C0134522101EPX000SRCSUM0001.HTM</a> |
| 61223 | AB Dor                   |                          |                            | Guedel+ 2001; Matranga+ 2005                    | <a href="http://www.ledas.ac.uk/data/2XMM/0537_0134521701_002/C0134521701EPX000SRCSUM0001.HTM">http://www.ledas.ac.uk/data/2XMM/0537_0134521701EPX000SRCSUM0001.HTM</a>                 |
| 61222 | AB Dor                   |                          |                            | Guedel+ 2001; Matranga+ 2005                    | <a href="http://www.ledas.ac.uk/data/2XMM/0185_0133120201_003/C0133120201EPX000SRCSUM0001.HTM">http://www.ledas.ac.uk/data/2XMM/0185_0133120201_003/C0133120201EPX000SRCSUM0001.HTM</a> |
| 61224 | AB Dor                   |                          |                            | Guedel+ 2001; Matranga+ 2005                    | <a href="http://www.ledas.ac.uk/data/2XMM/0162_0123720301_002/C0123720301EPX000SRCSUM0001.HTM">http://www.ledas.ac.uk/data/2XMM/0162_0123720301_002/C0123720301EPX000SRCSUM0001.HTM</a> |
| 61213 | AB Dor                   |                          |                            | Guedel+ 2001; Matranga+ 2005                    | <a href="http://www.ledas.ac.uk/data/2XMM/0605_0134522301_002/C0134522301EPX000SRCSUM0001.HTM">http://www.ledas.ac.uk/data/2XMM/0605_0134522301_002/C0134522301EPX000SRCSUM0001.HTM</a> |
| 61219 | AB Dor                   |                          |                            | Guedel+ 2001; Matranga+ 2005                    | <a href="http://www.ledas.ac.uk/data/2XMM/0462_0134521601_002/C0134521601EPX000SRCSUM0001.HTM">http://www.ledas.ac.uk/data/2XMM/0462_0134521601_002/C0134521601EPX000SRCSUM0001.HTM</a> |
| 61221 | AB Dor                   |                          |                            | Guedel+ 2001; Matranga+ 2005                    | <a href="http://www.ledas.ac.uk/data/2XMM/0709_0160362701_002/C0160362701EPX000SRCSUM0001.HTM">http://www.ledas.ac.uk/data/2XMM/0709_0160362701_002/C0160362701EPX000SRCSUM0001.HTM</a> |
| 61220 | AB Dor                   |                          |                            | Guedel+ 2001; Matranga+ 2005                    | <a href="http://www.ledas.ac.uk/data/2XMM/0546_0134522001_002/C0134522001EPX000SRCSUM0001.HTM">http://www.ledas.ac.uk/data/2XMM/0546_0134522001_002/C0134522001EPX000SRCSUM0001.HTM</a> |
| 64214 | 2MASS J05350341-0505402  | in OMC-2/3?              |                            |                                                 | <a href="http://www.ledas.ac.uk/data/2XMM/0598_0134531601_003/C0134531601EPX000SRCSUM0028.HTM">http://www.ledas.ac.uk/data/2XMM/0598_0134531601_003/C0134531601EPX000SRCSUM0028.HTM</a> |
| 65197 | HD 37040                 |                          |                            | Naze 2009                                       | <a href="http://www.ledas.ac.uk/data/2XMM/0507_0049560301_002/C0049560301EPX000SRCSUM0007.HTM">http://www.ledas.ac.uk/data/2XMM/0507_0049560301_002/C0049560301EPX000SRCSUM0007.HTM</a> |
| 71057 | chi01 Ori                |                          |                            | Telleschi+ 2005                                 | <a href="http://www.ledas.ac.uk/data/2XMM/0243_0111500101_002/C0111500101EPX000SRCSUM0001.HTM">http://www.ledas.ac.uk/data/2XMM/0243_0111500101_002/C0111500101EPX000SRCSUM0001.HTM</a> |
| 75409 | SV Cam                   | period ~0.59 dy          |                            | Sanz-Forcada+ 2006                              | <a href="http://www.ledas.ac.uk/data/2XMM/0238_0029340101_003/C0029340101EPX000SRCSUM0001.HTM">http://www.ledas.ac.uk/data/2XMM/0238_0029340101_003/C0029340101EPX000SRCSUM0001.HTM</a> |
| 75410 | SV Cam                   | period ~0.59 dy          |                            | Sanz-Forcada+ 2006                              | <a href="http://www.ledas.ac.uk/data/2XMM/0700_0029340201_002/C0029340201EPX000SRCSUM0001.HTM">http://www.ledas.ac.uk/data/2XMM/0700_0029340201_002/C0029340201EPX000SRCSUM0001.HTM</a> |
| 79319 | HD 51141                 |                          |                            |                                                 | <a href="http://www.ledas.ac.uk/data/2XMM/0232_0022340201_002/C0022340201EPX000SRCSUM0009.HTM">http://www.ledas.ac.uk/data/2XMM/0232_0022340201_002/C0022340201EPX000SRCSUM0009.HTM</a> |
| 80086 | HD 59581                 | period ~2.3 dy           | Stocke+ 1991; Favata+ 1995 |                                                 | <a href="http://www.ledas.ac.uk/data/2XMM/0872_0164560901_001/C0164560901EPX000SRCSUM0003.HTM">http://www.ledas.ac.uk/data/2XMM/0872_0164560901_001/C0164560901EPX000SRCSUM0003.HTM</a> |
| 81491 | YZ CMI                   |                          |                            |                                                 | <a href="http://www.ledas.ac.uk/data/2XMM/0153_0111460101_002/C0111460101EPX000SRCSUM0001.HTM">http://www.ledas.ac.uk/data/2XMM/0153_0111460101_002/C0111460101EPX000SRCSUM0001.HTM</a> |
| 89993 | 2MASS J08322856+5245330  |                          |                            | Mitra-Kraev+ 2005a; Smith+ 2005; Raassen+ 2007  | <a href="http://www.ledas.ac.uk/data/2XMM/0437_0092800201_003/C0092800201EPX000SRCSUM000F.HTM">http://www.ledas.ac.uk/data/2XMM/0437_0092800201_003/C0092800201EPX000SRCSUM000F.HTM</a> |
| 91247 | pi.01 UMa                |                          |                            | Telleschi+ 2005                                 | <a href="http://www.ledas.ac.uk/data/2XMM/0166_0111400101_002/C0111400101EPX000SRCSUM0001.HTM">http://www.ledas.ac.uk/data/2XMM/0166_0111400101_002/C0111400101EPX000SRCSUM0001.HTM</a> |
| 91420 | HD 73709                 | in Praesepe open cluster |                            | Franciosini+ 2003                               | <a href="http://www.ledas.ac.uk/data/2XMM/0168_0101440401_002/C0101440401EPX000SRCSUM001A.HTM">http://www.ledas.ac.uk/data/2XMM/0168_0101440401_002/C0101440401EPX000SRCSUM001A.HTM</a> |

| DETID  | Star_Name               | Star_Notes                                      | Star_Ref                      | XMM_Ref                                                         | DPsummaryLink                                                                                                                                                                           |
|--------|-------------------------|-------------------------------------------------|-------------------------------|-----------------------------------------------------------------|-----------------------------------------------------------------------------------------------------------------------------------------------------------------------------------------|
| 93362  | CD-45 4602              | period ~0.48 dy                                 | Pribulla+ 2001                |                                                                 | <a href="http://www.ledas.ac.uk/data/2XMM/0718_0162360101_003/C0162360101EPX000SRCSUM0003.HTM">http://www.ledas.ac.uk/data/2XMM/0718_0162360101_003/C0162360101EPX000SRCSUM0003.HTM</a> |
| 93359  | CD-45 4602              |                                                 |                               |                                                                 | <a href="http://www.ledas.ac.uk/data/2XMM/0252_0112870301_002/C0112870301EPX000SRCSUM0004.HTM">http://www.ledas.ac.uk/data/2XMM/0252_0112870301_002/C0112870301EPX000SRCSUM0004.HTM</a> |
| 95682  | XY UMa                  |                                                 |                               |                                                                 | <a href="http://www.ledas.ac.uk/data/2XMM/0971_0200960101_001/C0200960101EPX000SRCSUM0001.HTM">http://www.ledas.ac.uk/data/2XMM/0971_0200960101_001/C0200960101EPX000SRCSUM0001.HTM</a> |
| 98763  | LQ Hya                  |                                                 |                               |                                                                 | <a href="http://www.ledas.ac.uk/data/2XMM/0625_0148880101_002/C0148880101EPX000SRCSUM0001.HTM">http://www.ledas.ac.uk/data/2XMM/0625_0148880101_002/C0148880101EPX000SRCSUM0001.HTM</a> |
| 98764  | LQ Hya                  |                                                 |                               |                                                                 | <a href="http://www.ledas.ac.uk/data/2XMM/0724_0148880301_002/C0148880301EPX000SRCSUM0001.HTM">http://www.ledas.ac.uk/data/2XMM/0724_0148880301_002/C0148880301EPX000SRCSUM0001.HTM</a> |
| 99591  | HD 83698                | in Lockman Deep Field                           | Otero+ 2004; Griffin 2009     | van den Besselaar+ 2003; Robrade+ 2005; Smith+ 2005             | <a href="http://www.ledas.ac.uk/data/2XMM/0813_0203270101_001/C0203270101EPX000SRCSUM0002.HTM">http://www.ledas.ac.uk/data/2XMM/0813_0203270101_001/C0203270101EPX000SRCSUM0002.HTM</a> |
| 101535 | 2MASS J09553615+6954487 |                                                 |                               |                                                                 | <a href="http://www.ledas.ac.uk/data/2XMM/0800_0206080101_001/C0206080101EPX000SRCSUM0012.HTM">http://www.ledas.ac.uk/data/2XMM/0800_0206080101_001/C0206080101EPX000SRCSUM0012.HTM</a> |
| 108025 | AD Leo                  |                                                 |                               |                                                                 | <a href="http://www.ledas.ac.uk/data/2XMM/0262_011440101_002/C011440101EPX000SRCSUM0001.HTM">http://www.ledas.ac.uk/data/2XMM/0262_011440101_002/C011440101EPX000SRCSUM0001.HTM</a>     |
| 118876 | NU UMa                  |                                                 |                               |                                                                 | <a href="http://www.ledas.ac.uk/data/2XMM/0544_0147511601_002/C0147511601EPX000SRCSUM0005.HTM">http://www.ledas.ac.uk/data/2XMM/0544_0147511601_002/C0147511601EPX000SRCSUM0005.HTM</a> |
| 120401 | CR Cha                  |                                                 |                               |                                                                 | <a href="http://www.ledas.ac.uk/data/2XMM/0222_0067140201_002/C0067140201EPX000SRCSUM0001.HTM">http://www.ledas.ac.uk/data/2XMM/0222_0067140201_002/C0067140201EPX000SRCSUM0001.HTM</a> |
| 121057 | HD 95735                | has possible exoplanet                          |                               | Robrade+ 2006                                                   | <a href="http://www.ledas.ac.uk/data/2XMM/0810_0205370101_002/C0205370101EPX000SRCSUM0001.HTM">http://www.ledas.ac.uk/data/2XMM/0810_0205370101_002/C0205370101EPX000SRCSUM0001.HTM</a> |
| 123749 | GSC 09414-00787         | in stellar association Cha T 2-21               |                               | Lopez-Santiago+ 2007                                            | <a href="http://www.ledas.ac.uk/data/2XMM/0773_0203810201_002/C0203810201EPX000SRCSUM0001.HTM">http://www.ledas.ac.uk/data/2XMM/0773_0203810201_002/C0203810201EPX000SRCSUM0001.HTM</a> |
| 130963 | HD 104021               | in stellar cluster Sco OB2                      |                               | Stelzer+ 2004                                                   | <a href="http://www.ledas.ac.uk/data/2XMM/1111_0301430101_001/C0301430101EPX000SRCSUM0001.HTM">http://www.ledas.ac.uk/data/2XMM/1111_0301430101_001/C0301430101EPX000SRCSUM0001.HTM</a> |
| 142357 | HD 108984               |                                                 |                               |                                                                 | <a href="http://www.ledas.ac.uk/data/2XMM/1022_0301450201_002/C0301450201EPX000SRCSUM0002.HTM">http://www.ledas.ac.uk/data/2XMM/1022_0301450201_002/C0301450201EPX000SRCSUM0002.HTM</a> |
| 148010 | IM Vir                  |                                                 | Pourbaix+ 2004; Morales+ 2009 | Pandey+ 2008; Lopez-Santiago+ 2007                              | <a href="http://www.ledas.ac.uk/data/2XMM/0842_0203270301_001/C0203270301EPX000SRCSUM0001.HTM">http://www.ledas.ac.uk/data/2XMM/0842_0203270301_001/C0203270301EPX000SRCSUM0001.HTM</a> |
| 148011 | IM Vir                  |                                                 | Pourbaix+ 2004; Morales+ 2009 | Pandey+ 2008; Lopez-Santiago+ 2007                              | <a href="http://www.ledas.ac.uk/data/2XMM/0291_0060370201_002/C0060370201EPX000SRCSUM0001.HTM">http://www.ledas.ac.uk/data/2XMM/0291_0060370201_002/C0060370201EPX000SRCSUM0001.HTM</a> |
| 156921 | 2MASS J13141103-1620235 |                                                 |                               |                                                                 | <a href="http://www.ledas.ac.uk/data/2XMM/1113_0301290101_001/C0301290101EPX000SRCSUM0004.HTM">http://www.ledas.ac.uk/data/2XMM/1113_0301290101_001/C0301290101EPX000SRCSUM0004.HTM</a> |
| 160700 | FK Com                  |                                                 |                               | Gondoin+ 2002                                                   | <a href="http://www.ledas.ac.uk/data/2XMM/0205_0100240201_002/C0100240201EPX000SRCSUM0001.HTM">http://www.ledas.ac.uk/data/2XMM/0205_0100240201_002/C0100240201EPX000SRCSUM0001.HTM</a> |
| 160701 | FK Com                  |                                                 |                               | Gondoin+ 2002                                                   | <a href="http://www.ledas.ac.uk/data/2XMM/0199_0100240101_002/C0100240101EPX000SRCSUM0001.HTM">http://www.ledas.ac.uk/data/2XMM/0199_0100240101_002/C0100240101EPX000SRCSUM0001.HTM</a> |
| 161095 | DG CVn                  |                                                 |                               |                                                                 | <a href="http://www.ledas.ac.uk/data/2XMM/1104_0301040101_001/C0301040101EPX000SRCSUM0001.HTM">http://www.ledas.ac.uk/data/2XMM/1104_0301040101_001/C0301040101EPX000SRCSUM0001.HTM</a> |
| 163132 | 2MASS J13362690-3426365 |                                                 |                               | Lopez-Santiago+ 2007                                            | <a href="http://www.ledas.ac.uk/data/2XMM/0301_0029740101_002/C0029740101EPX000SRCSUM0002.HTM">http://www.ledas.ac.uk/data/2XMM/0301_0029740101_002/C0029740101EPX000SRCSUM0002.HTM</a> |
| 165709 | tau Boo                 | has exoplanet                                   |                               | Maggio+ 2011                                                    | <a href="http://www.ledas.ac.uk/data/2XMM/0648_0144570101_003/C0144570101EPX000SRCSUM0001.HTM">http://www.ledas.ac.uk/data/2XMM/0648_0144570101_003/C0144570101EPX000SRCSUM0001.HTM</a> |
| 169401 | HD 122473               |                                                 |                               | Lopez-Santiago+ 2007                                            | <a href="http://www.ledas.ac.uk/data/2XMM/0200_0109910101_004/C0109910101EPX000SRCSUM0007.HTM">http://www.ledas.ac.uk/data/2XMM/0200_0109910101_004/C0109910101EPX000SRCSUM0007.HTM</a> |
| 170306 | GSC 03852-01069         | in M101 field                                   |                               |                                                                 | <a href="http://www.ledas.ac.uk/data/2XMM/0931_0212480201_001/C0212480201EPX000SRCSUM0004.HTM">http://www.ledas.ac.uk/data/2XMM/0931_0212480201_001/C0212480201EPX000SRCSUM0004.HTM</a> |
| 174625 | HD 127244               |                                                 |                               | Lopez-Santiago+ 2007                                            | <a href="http://www.ledas.ac.uk/data/2XMM/1012_0310190101_002/C0310190101EPX000SRCSUM0005.HTM">http://www.ledas.ac.uk/data/2XMM/1012_0310190101_002/C0310190101EPX000SRCSUM0005.HTM</a> |
| 175724 | EK Dra                  |                                                 |                               | Scelsi+ 2005; Telleschi+ 2005; Nordon+ 2008                     | <a href="http://www.ledas.ac.uk/data/2XMM/0194_0111530101_002/C0111530101EPX000SRCSUM0001.HTM">http://www.ledas.ac.uk/data/2XMM/0194_0111530101_002/C0111530101EPX000SRCSUM0001.HTM</a> |
| 177789 | xi Boo A                |                                                 |                               | Nordon+ 2008; Pandey+ 2008                                      | <a href="http://www.ledas.ac.uk/data/2XMM/0204_0056030101_002/C0056030101EPX000SRCSUM0001.HTM">http://www.ledas.ac.uk/data/2XMM/0204_0056030101_002/C0056030101EPX000SRCSUM0001.HTM</a> |
| 179597 | 44 Boo                  |                                                 |                               | Gondoin+ 2004b                                                  | <a href="http://www.ledas.ac.uk/data/2XMM/0274_0100650101_003/C0100650101EPX000SRCSUM0001.HTM">http://www.ledas.ac.uk/data/2XMM/0274_0100650101_003/C0100650101EPX000SRCSUM0001.HTM</a> |
| 182638 | UZ Lib                  |                                                 |                               | Gondoin+ 2003; Pandey+ 2012                                     | <a href="http://www.ledas.ac.uk/data/2XMM/0210_0100240801_002/C0100240801EPX000SRCSUM0001.HTM">http://www.ledas.ac.uk/data/2XMM/0210_0100240801_002/C0100240801EPX000SRCSUM0001.HTM</a> |
| 187347 | sigma*2 CrB             |                                                 |                               | Suh+ 2005                                                       | <a href="http://www.ledas.ac.uk/data/2XMM/0404_0111470301_002/C0111470301EPX000SRCSUM0001.HTM">http://www.ledas.ac.uk/data/2XMM/0404_0111470301_002/C0111470301EPX000SRCSUM0001.HTM</a> |
| 193025 | CD-53 6825              | in wings of bright X-ray source (X1636-536)     |                               |                                                                 | <a href="http://www.ledas.ac.uk/data/2XMM/0313_0105470401_003/C0105470401EPX000SRCSUM0001.HTM">http://www.ledas.ac.uk/data/2XMM/0313_0105470401_003/C0105470401EPX000SRCSUM0001.HTM</a> |
| 194097 | alf TrA                 | "hybrid chromosphere"-type star; +dG companion? | Ayres 2005; Ayres+ 2007       |                                                                 | <a href="http://www.ledas.ac.uk/data/2XMM/0226_0021750501_002/C0021750501EPX000SRCSUM0001.HTM">http://www.ledas.ac.uk/data/2XMM/0226_0021750501_002/C0021750501EPX000SRCSUM0001.HTM</a> |
| 194425 | TYC 9275-01654-1        |                                                 |                               |                                                                 | <a href="http://www.ledas.ac.uk/data/2XMM/0226_0021750701_002/C0021750701EPX000SRCSUM0003.HTM">http://www.ledas.ac.uk/data/2XMM/0226_0021750701_002/C0021750701EPX000SRCSUM0003.HTM</a> |
| 204777 | BN Sgr                  |                                                 | Malkov+ 2006                  |                                                                 | <a href="http://www.ledas.ac.uk/data/2XMM/0145_0112970201_003/C0112970201EPX000SRCSUM0001.HTM">http://www.ledas.ac.uk/data/2XMM/0145_0112970201_003/C0112970201EPX000SRCSUM0001.HTM</a> |
| 210451 | 70 Oph                  | binary separation~5"                            |                               |                                                                 | <a href="http://www.ledas.ac.uk/data/2XMM/0688_0044741301_002/C0044741301EPX000SRCSUM0001.HTM">http://www.ledas.ac.uk/data/2XMM/0688_0044741301_002/C0044741301EPX000SRCSUM0001.HTM</a> |
| 212517 | HD 166191               |                                                 |                               |                                                                 | <a href="http://www.ledas.ac.uk/data/2XMM/0882_0201270101_001/C0201270101EPX000SRCSUM0003.HTM">http://www.ledas.ac.uk/data/2XMM/0882_0201270101_001/C0201270101EPX000SRCSUM0003.HTM</a> |
| 217384 | 2MASS J18403031+0513166 |                                                 |                               |                                                                 | <a href="http://www.ledas.ac.uk/data/2XMM/0787_0084020601_002/C0084020601EPX000SRCSUM0002.HTM">http://www.ledas.ac.uk/data/2XMM/0787_0084020601_002/C0084020601EPX000SRCSUM0002.HTM</a> |
| 219667 | V709 CrA                |                                                 |                               |                                                                 | <a href="http://www.ledas.ac.uk/data/2XMM/0604_0146390101_002/C0146390101EPX000SRCSUM0002.HTM">http://www.ledas.ac.uk/data/2XMM/0604_0146390101_002/C0146390101EPX000SRCSUM0002.HTM</a> |
| 224075 | TYC 1082-02107-1        |                                                 |                               |                                                                 | <a href="http://www.ledas.ac.uk/data/2XMM/0526_0112960501_002/C0112960501EPX000SRCSUM0001.HTM">http://www.ledas.ac.uk/data/2XMM/0526_0112960501_002/C0112960501EPX000SRCSUM0001.HTM</a> |
| 226652 | VW Cep                  |                                                 |                               | Gondoin+ 2004a                                                  | <a href="http://www.ledas.ac.uk/data/2XMM/0529_0100650301_003/C0100650301EPX000SRCSUM0001.HTM">http://www.ledas.ac.uk/data/2XMM/0529_0100650301_003/C0100650301EPX000SRCSUM0001.HTM</a> |
| 226653 | VW Cep                  |                                                 |                               | Gondoin+ 2004a                                                  | <a href="http://www.ledas.ac.uk/data/2XMM/0515_0100650201_002/C0100650201EPX000SRCSUM0001.HTM">http://www.ledas.ac.uk/data/2XMM/0515_0100650201_002/C0100650201EPX000SRCSUM0001.HTM</a> |
| 226922 | AT Mic                  |                                                 |                               | Raassen+ 2003; Mitra-Kraev+ 2005a,b; Robrade+ 2005; Smith+ 2005 | <a href="http://www.ledas.ac.uk/data/2XMM/0156_0111510101_003/C0111510101EPX000SRCSUM0001.HTM">http://www.ledas.ac.uk/data/2XMM/0156_0111510101_003/C0111510101EPX000SRCSUM0001.HTM</a> |
| 227252 | AU Mic                  |                                                 |                               | Mitra-Kraev+ 2005a; Smith+ 2005                                 | <a href="http://www.ledas.ac.uk/data/2XMM/0155_0111420101_003/C0111420101EPX000SRCSUM0001.HTM">http://www.ledas.ac.uk/data/2XMM/0155_0111420101_003/C0111420101EPX000SRCSUM0001.HTM</a> |
| 229724 | 61 Cyg A                |                                                 |                               | Hempelmann+ 2006                                                | <a href="http://www.ledas.ac.uk/data/2XMM/0724_0041741001_002/C0041741001EPX000SRCSUM0001.HTM">http://www.ledas.ac.uk/data/2XMM/0724_0041741001_002/C0041741001EPX000SRCSUM0001.HTM</a> |
| 229734 | 61 Cyg B                |                                                 |                               | Hempelmann+ 2006                                                | <a href="http://www.ledas.ac.uk/data/2XMM/0805_0041741101_002/C0041741101EPX000SRCSUM0002.HTM">http://www.ledas.ac.uk/data/2XMM/0805_0041741101_002/C0041741101EPX000SRCSUM0002.HTM</a> |
| 229736 | 61 Cyg B                |                                                 |                               | Hempelmann+ 2006                                                | <a href="http://www.ledas.ac.uk/data/2XMM/0898_0143630101_001/C0143630101EPX000SRCSUM0001.HTM">http://www.ledas.ac.uk/data/2XMM/0898_0143630101_001/C0143630101EPX000SRCSUM0001.HTM</a> |
| 231002 | SAO 10050               |                                                 |                               |                                                                 | <a href="http://www.ledas.ac.uk/data/2XMM/1036_0300490501_001/C0300490501EPX000SRCSUM0002.HTM">http://www.ledas.ac.uk/data/2XMM/1036_0300490501_001/C0300490501EPX000SRCSUM0002.HTM</a> |
| 239075 | EV Lac                  |                                                 |                               | Mitra-Kraev+ 2005a; Robrade+ 2005                               | <a href="http://www.ledas.ac.uk/data/2XMM/0272_0111450101_002/C0111450101EPX000SRCSUM0001.HTM">http://www.ledas.ac.uk/data/2XMM/0272_0111450101_002/C0111450101EPX000SRCSUM0001.HTM</a> |
| 241508 | HK Aqr                  |                                                 |                               |                                                                 | <a href="http://www.ledas.ac.uk/data/2XMM/0996_0202360101_001/C0202360101EPX000SRCSUM0001.HTM">http://www.ledas.ac.uk/data/2XMM/0996_0202360101_001/C0202360101EPX000SRCSUM0001.HTM</a> |
| 242179 | 1RXS J231628.7+790531   |                                                 |                               |                                                                 | <a href="http://www.ledas.ac.uk/data/2XMM/0742_0203060101_003/C0203060101EPX000SRCSUM0002.HTM">http://www.ledas.ac.uk/data/2XMM/0742_0203060101_003/C0203060101EPX000SRCSUM0002.HTM</a> |
| 242641 | V368 Cep                |                                                 |                               |                                                                 | <a href="http://www.ledas.ac.uk/data/2XMM/0742_0203060101_003/C0203060101EPX000SRCSUM0001.HTM">http://www.ledas.ac.uk/data/2XMM/0742_0203060101_003/C0203060101EPX000SRCSUM0001.HTM</a> |
| 243984 | EQ Peg                  |                                                 |                               | Pandey+ 2008                                                    | <a href="http://www.ledas.ac.uk/data/2XMM/0107_0112880301_004/C0112880301EPX000SRCSUM0001.HTM">http://www.ledas.ac.uk/data/2XMM/0107_0112880301_004/C0112880301EPX000SRCSUM0001.HTM</a> |
| 243985 | EQ Peg                  |                                                 |                               | Robrade+ 2004, 2005                                             | <a href="http://www.ledas.ac.uk/data/2XMM/0559_0147580301_002/C0147580301EPX000SRCSUM0001.HTM">http://www.ledas.ac.uk/data/2XMM/0559_0147580301_002/C0147580301EPX000SRCSUM0001.HTM</a> |
| 244744 | Iam And                 |                                                 |                               | Audard+ 2003; Pandey+ 2012                                      | <a href="http://www.ledas.ac.uk/data/2XMM/0208_0099320101_002/C0099320101EPX000SRCSUM0001.HTM">http://www.ledas.ac.uk/data/2XMM/0208_0099320101_002/C0099320101EPX000SRCSUM0001.HTM</a> |

| Column Name   | Description                                                                                                                                                                                              | Units        | Origin                                                                                                                                                                                                                                                                                                                                                                                                                                         |
|---------------|----------------------------------------------------------------------------------------------------------------------------------------------------------------------------------------------------------|--------------|------------------------------------------------------------------------------------------------------------------------------------------------------------------------------------------------------------------------------------------------------------------------------------------------------------------------------------------------------------------------------------------------------------------------------------------------|
| DETID         | a consecutive number which identifies each entry (detection) in the 2XMM catalogue                                                                                                                       |              | 2XMM                                                                                                                                                                                                                                                                                                                                                                                                                                           |
| Star_Name     | identifying name for the star                                                                                                                                                                            |              | SIMBAD+                                                                                                                                                                                                                                                                                                                                                                                                                                        |
| Alt_Name      | additional identifying name for the star                                                                                                                                                                 |              | SIMBAD+                                                                                                                                                                                                                                                                                                                                                                                                                                        |
| TychoId       | star's identifier in the Tycho-2 catalogue                                                                                                                                                               |              | Tycho-2                                                                                                                                                                                                                                                                                                                                                                                                                                        |
| Vmag          | star's V-band apparent magnitude, see Sect. 2.4                                                                                                                                                          |              | Tycho-2 derived                                                                                                                                                                                                                                                                                                                                                                                                                                |
| B-V           | star's B-V colour, uncorrected for redenning, see Sect. 2.4                                                                                                                                              |              | Tycho-2 derived                                                                                                                                                                                                                                                                                                                                                                                                                                |
| Star_SpType   | star's spectral type, e.g. G2 V                                                                                                                                                                          |              | SIMBAD+                                                                                                                                                                                                                                                                                                                                                                                                                                        |
| Star_Type     | star's type, category or characteristics, e.g. RS CVn-type. EB = eclipsing binary, SB = spectroscopic binary, SB1 = single-lined SB, PMS = pre-main-sequence star                                        |              | SIMBAD+                                                                                                                                                                                                                                                                                                                                                                                                                                        |
| Dist          | distance to star, from Earth                                                                                                                                                                             | pc           | see DistRef                                                                                                                                                                                                                                                                                                                                                                                                                                    |
| DistRef       | source of distance value                                                                                                                                                                                 |              | HIP=Hipparcos (van Leeuwen 2007), TYC=Tycho (ph.par. from V, see Sect.2.4), N2K=Ammons et al. 2006, GCT=van Altena et al. 1995, B04=Budding et al. 2004, F03=Favata et al. 2003, F07=Franciosi et al. 2007a, F95=Favata et al. 1995, G07=Guedel et al. 2007a, M09=Morales et al. 2009, M81=Marraco et al. 1981, R95=Reid et al. 1995, R99=Robichon et al. 1999, S04=Stelzer et al. 2004, T02=Tsujiimoto et al. 2002, Z04=Zuckerman et al. 2004 |
| OBS_TARGET    | = TRUE if source/star is considered to be the target of the observation                                                                                                                                  |              | 2XMM                                                                                                                                                                                                                                                                                                                                                                                                                                           |
| CoolVflag     | = TRUE if considered to be a good, cool-star, variable detection in 2XMM (i.e. in CVS sample); = FALSE if in "low-variability" (CLVS) sample; see Sect. 3                                                |              | this work                                                                                                                                                                                                                                                                                                                                                                                                                                      |
| SRCID         | a unique number assigned to a group of 2XMM catalogue entries (DETIDs) which are assumed to be the same                                                                                                  |              | 2XMM                                                                                                                                                                                                                                                                                                                                                                                                                                           |
| SrcIdOther    | indicates if SRCID should be matched to another SRCID, see Sect 2.3; relates to high-proper-motion stars                                                                                                 |              | 2XMM derived                                                                                                                                                                                                                                                                                                                                                                                                                                   |
| IAUNAME       | the IAU name assigned to the unique SRCID                                                                                                                                                                |              | 2XMM                                                                                                                                                                                                                                                                                                                                                                                                                                           |
| logFxFv       | log10 (total-band [0.2-12 keV] 2XMM flux / visual-band Tycho-2 flux)                                                                                                                                     |              | 2XMM+Tycho-2 derived                                                                                                                                                                                                                                                                                                                                                                                                                           |
| logLx         | log10 (total-band [0.2-12 keV] X-ray luminosity)                                                                                                                                                         | log10(erg/s) | 2XMM+Tycho-2+Dist derived                                                                                                                                                                                                                                                                                                                                                                                                                      |
| OBS_ID        | the XMM-Newton observation identification                                                                                                                                                                |              | 2XMM                                                                                                                                                                                                                                                                                                                                                                                                                                           |
| Tsfile        | name of 2XMM time-series (i.e. light-curve) file (minus file-type extension)                                                                                                                             |              | 2XMM                                                                                                                                                                                                                                                                                                                                                                                                                                           |
| MJD_START     | modified Julian Date (i.e. JD-2 400 000.5) of the start of the observation                                                                                                                               | d            | 2XMM                                                                                                                                                                                                                                                                                                                                                                                                                                           |
| MJD_STOP      | modified Julian Date (i.e. JD-2 400 000.5) of the end of the observation                                                                                                                                 | d            | 2XMM                                                                                                                                                                                                                                                                                                                                                                                                                                           |
| OnTime        | M1_ONTIME if available, else M2_ONTIME, else PN_ONTIME; where ca_ONTIME is the total good exposure time (after GTI filtering) for the detection                                                          | s            | 2XMM derived                                                                                                                                                                                                                                                                                                                                                                                                                                   |
| PN_FILTER     | optical blocking filter used in PN camera                                                                                                                                                                |              | 2XMM                                                                                                                                                                                                                                                                                                                                                                                                                                           |
| M1_FILTER     | optical blocking filter used in M1 camera                                                                                                                                                                |              | 2XMM                                                                                                                                                                                                                                                                                                                                                                                                                                           |
| M2_FILTER     | optical blocking filter used in M2 camera                                                                                                                                                                |              | 2XMM                                                                                                                                                                                                                                                                                                                                                                                                                                           |
| OFFAX_MIN     | min (PN_OFFAX, M1_OFFAX, M2_OFFAX); where ca_OFFAX is the off-axis angle of the source                                                                                                                   | arcmin       | 2XMM derived                                                                                                                                                                                                                                                                                                                                                                                                                                   |
| VAR_INST_ID   | instrument (PN, M1, M2) corresponding to the exposure with the lowest variability chi-square probability                                                                                                 |              | 2XMM                                                                                                                                                                                                                                                                                                                                                                                                                                           |
| SUM_FLAG2     | summary "quality" flag for the detection, based on 2XMM SUM_FLAG, but re-evaluated for present work; =6 if counting-mode exposure problems; =5 if optical loading; =-3 if flag12=T; else = 2XMM SUM_FLAG |              | 2XMM derived                                                                                                                                                                                                                                                                                                                                                                                                                                   |
| NrEvents      | number of flares or other "events" identified in the light-curve                                                                                                                                         |              | this work                                                                                                                                                                                                                                                                                                                                                                                                                                      |
| Star_Notes    | notes on star's properties etc                                                                                                                                                                           |              | this work                                                                                                                                                                                                                                                                                                                                                                                                                                      |
| Star_Ref      | selected reference(s) relating to star                                                                                                                                                                   |              | this work                                                                                                                                                                                                                                                                                                                                                                                                                                      |
| XMM_Ref       | reference(s) reporting relevant XMM-Newton results                                                                                                                                                       |              | this work                                                                                                                                                                                                                                                                                                                                                                                                                                      |
| DPsummaryLink | URL link to 2XMM summary-results web page at LEDAS                                                                                                                                                       |              | 2XMM derived                                                                                                                                                                                                                                                                                                                                                                                                                                   |
| <b>NOTES:</b> |                                                                                                                                                                                                          |              |                                                                                                                                                                                                                                                                                                                                                                                                                                                |
| Description:  | for parameters from 2XMM & Tycho-2, more information may be found in those catalogues                                                                                                                    |              |                                                                                                                                                                                                                                                                                                                                                                                                                                                |
| Origin:       | 2XMM/Tycho-2 = values taken directly from 2XMM/Tycho-2 catalogue<br>2XMM/Tycho-2 derived = based on values in 2XMM/Tycho-2 catalogue<br>SIMBAD+ = taken from CDS SIMBAD database and other sources       |              |                                                                                                                                                                                                                                                                                                                                                                                                                                                |
