# Supplementary material for: A survey of stellar X-ray flares from the XMM-Newton serendipitous source catalogue: Hipparcos-Tycho cool stars
Source: arXiv:1506.05289 ancillary file (2015-06-17)
Supplement: Supplementary file 2 [file Table-C.2-VarParams-ElOnly-v03.pdf]

| DETID | EventNr | SRCID | Star_Name                | ProfileFlag | FlareFlag | EventType     | SNR   | fx_quies | fx_peak  | r_peak | quies_t_peak | dt_rise | dt_fall | dt_duration | Lx_quies | Lx_peak  | Ex       | DpsummaryLink                                                                                                                                                                           |
|-------|---------|-------|--------------------------|-------------|-----------|---------------|-------|----------|----------|--------|--------------|---------|---------|-------------|----------|----------|----------|-----------------------------------------------------------------------------------------------------------------------------------------------------------------------------------------|
| 1916  | 1       | 1821  | UV Scl                   | TRUE        | FALSE     | indeterminate | 15.4  | 3.55E-13 | 2.24E-13 | 0.6    | 17280        | 7830    | 5400    | 13230       | 7.99E+29 | 5.03E+29 | 4.19E+33 | <a href="http://www.ledas.ac.uk/data/2XMM/0354_0028740101_002/C0028740101EPX000SRCSUM0003.HTM">http://www.ledas.ac.uk/data/2XMM/0354_0028740101_002/C0028740101EPX000SRCSUM0003.HTM</a> |
| 2236  | 1       | 2107  | HD 1165                  | TRUE        | TRUE      | flare         | 5.5   | 2.82E-13 | 4.90E-13 | 1.7    | 13440        | 320     | 960     | 1280        | 3.72E+28 | 6.46E+28 | 6.17E+31 | <a href="http://www.ledas.ac.uk/data/2XMM/0312_0112620201_003/C0112620201EPX000SRCSUM0002.HTM">http://www.ledas.ac.uk/data/2XMM/0312_0112620201_003/C0112620201EPX000SRCSUM0002.HTM</a> |
| 15656 | 1       | 12024 | HD 8191                  | TRUE        | TRUE      | flare         | 6.1   | 6.77E-13 | 2.14E-13 | 0.3    | 37240        | 910     | 2870    | 3780        | 1.05E+29 | 3.31E+28 | 8.36E+31 | <a href="http://www.ledas.ac.uk/data/2XMM/0270_0011450101_002/C0011450101EPX000SRCSUM0002.HTM">http://www.ledas.ac.uk/data/2XMM/0270_0011450101_002/C0011450101EPX000SRCSUM0002.HTM</a> |
| 22001 | 1       | 17021 | 47 Cas B                 | TRUE        | TRUE      | flare         | 28.7  | 1.71E-11 | 1.62E-11 | 0.9    | 14230        | 610     | 1960    | 2570        | 2.24E+30 | 2.13E+30 | 3.01E+33 | <a href="http://www.ledas.ac.uk/data/2XMM/0322_0111520101_003/C0111520101EPX000SRCSUM0001.HTM">http://www.ledas.ac.uk/data/2XMM/0322_0111520101_003/C0111520101EPX000SRCSUM0001.HTM</a> |
| 23485 | 1       | 18148 | HD 14716                 | TRUE        | TRUE      | flare         | 43.6  | 1.41E-13 | 1.37E-12 | 9.7    | 21890        | 1760    | 5170    | 6930        | 6.48E+28 | 6.29E+29 | 2.84E+33 | <a href="http://www.ledas.ac.uk/data/2XMM/0876_0202130101_001/C0202130101EPX000SRCSUM0001.HTM">http://www.ledas.ac.uk/data/2XMM/0876_0202130101_001/C0202130101EPX000SRCSUM0001.HTM</a> |
| 30805 | 1       | 24119 | CC Eri                   | TRUE        | TRUE      | flare         | 23.6  | 2.00E-11 | 1.76E-11 | 0.9    | 10490        | 450     | 610     | 1060        | 3.22E+29 | 2.80E+29 | 2.16E+32 | <a href="http://www.ledas.ac.uk/data/2XMM/0671_0148790101_003/C0148790101EPX000SRCSUM0001.HTM">http://www.ledas.ac.uk/data/2XMM/0671_0148790101_003/C0148790101EPX000SRCSUM0001.HTM</a> |
| 30805 | 2       | 24119 | CC Eri                   | TRUE        | TRUE      | flare         | 44.0  | 2.03E-11 | 1.77E-11 | 0.9    | 29040        | 490     | 4440    | 4930        | 3.26E+29 | 2.86E+29 | 8.50E+32 | <a href="http://www.ledas.ac.uk/data/2XMM/0671_0148790101_003/C0148790101EPX000SRCSUM0001.HTM">http://www.ledas.ac.uk/data/2XMM/0671_0148790101_003/C0148790101EPX000SRCSUM0001.HTM</a> |
| 32470 | 1       | 25472 | CD-53 544                | TRUE        | TRUE      | flare         | 11.6  | 6.34E-12 | 4.85E-12 | 0.8    | 13890        | 600     | 970     | 1570        | 5.94E+29 | 4.55E+29 | 3.66E+32 | <a href="http://www.ledas.ac.uk/data/2XMM/0764_0207210101_002/C0207210101EPX000SRCSUM0001.HTM">http://www.ledas.ac.uk/data/2XMM/0764_0207210101_002/C0207210101EPX000SRCSUM0001.HTM</a> |
| 32470 | 2       | 25472 | CD-53 544                | TRUE        | TRUE      | flare         | 12.6  | 6.34E-12 | 4.76E-12 | 0.8    | 26190        | 450     | 1200    | 1650        | 5.94E+29 | 4.46E+29 | 4.10E+32 | <a href="http://www.ledas.ac.uk/data/2XMM/0764_0207210101_002/C0207210101EPX000SRCSUM0001.HTM">http://www.ledas.ac.uk/data/2XMM/0764_0207210101_002/C0207210101EPX000SRCSUM0001.HTM</a> |
| 32470 | 3       | 25472 | CD-53 544                | FALSE       | TRUE      | flare         | 36.3  | 6.34E-12 | 9.08E-12 | 1.4    | 34190        | 2340    | 1860    | 4200        | 5.94E+29 | 8.51E+29 | 2.17E+33 | <a href="http://www.ledas.ac.uk/data/2XMM/0764_0207210101_002/C0207210101EPX000SRCSUM0001.HTM">http://www.ledas.ac.uk/data/2XMM/0764_0207210101_002/C0207210101EPX000SRCSUM0001.HTM</a> |
| 33241 | 1       | 26140 | RZ Cas                   | TRUE        | TRUE      | flare         | 24.8  | 3.40E-12 | 5.65E-12 | 1.7    | 3960         | 1520    | 4030    | 5550        | 1.71E+30 | 2.83E+30 | 7.45E+33 | <a href="http://www.ledas.ac.uk/data/2XMM/0678_0149040201_002/C0149040201EPX000SRCSUM0001.HTM">http://www.ledas.ac.uk/data/2XMM/0678_0149040201_002/C0149040201EPX000SRCSUM0001.HTM</a> |
| 33241 | 2       | 26140 | RZ Cas                   | TRUE        | TRUE      | flare         | 15.3  | 3.40E-12 | 2.43E-12 | 0.7    | 65640        | 4160    | 3050    | 7210        | 1.71E+30 | 1.22E+30 | 4.53E+33 | <a href="http://www.ledas.ac.uk/data/2XMM/0678_0149040201_002/C0149040201EPX000SRCSUM0001.HTM">http://www.ledas.ac.uk/data/2XMM/0678_0149040201_002/C0149040201EPX000SRCSUM0001.HTM</a> |
| 33241 | 3       | 26140 | RZ Cas                   | TRUE        | TRUE      | flare         | 21.8  | 3.40E-12 | 3.20E-12 | 0.9    | 81990        | 3540    | 2410    | 5950        | 1.71E+30 | 1.60E+30 | 6.44E+33 | <a href="http://www.ledas.ac.uk/data/2XMM/0678_0149040201_002/C0149040201EPX000SRCSUM0001.HTM">http://www.ledas.ac.uk/data/2XMM/0678_0149040201_002/C0149040201EPX000SRCSUM0001.HTM</a> |
| 33241 | 4       | 26140 | RZ Cas                   | TRUE        | TRUE      | flare         | 18.7  | 3.40E-12 | 4.01E-12 | 1.2    | 101690       | 1100    | 1880    | 2980        | 1.71E+30 | 2.01E+30 | 4.18E+33 | <a href="http://www.ledas.ac.uk/data/2XMM/0678_0149040201_002/C0149040201EPX000SRCSUM0001.HTM">http://www.ledas.ac.uk/data/2XMM/0678_0149040201_002/C0149040201EPX000SRCSUM0001.HTM</a> |
| 33241 | 5       | 26140 | RZ Cas                   | TRUE        | TRUE      | flare         | 25.3  | 3.40E-12 | 5.18E-12 | 1.5    | 107740       | 1940    | 1470    | 3410        | 1.71E+30 | 2.60E+30 | 6.29E+33 | <a href="http://www.ledas.ac.uk/data/2XMM/0678_0149040201_002/C0149040201EPX000SRCSUM0001.HTM">http://www.ledas.ac.uk/data/2XMM/0678_0149040201_002/C0149040201EPX000SRCSUM0001.HTM</a> |
| 33241 | 6       | 26140 | RZ Cas                   | TRUE        | TRUE      | flare         | 26.7  | 3.40E-12 | 4.90E-12 | 1.4    | 112690       | 1670    | 1110    | 2780        | 1.71E+30 | 2.46E+30 | 6.42E+33 | <a href="http://www.ledas.ac.uk/data/2XMM/0678_0149040201_002/C0149040201EPX000SRCSUM0001.HTM">http://www.ledas.ac.uk/data/2XMM/0678_0149040201_002/C0149040201EPX000SRCSUM0001.HTM</a> |
| 37553 | 1       | 29517 | kap01 Cet                | TRUE        | TRUE      | flare         | 17.9  | 7.52E-12 | 6.03E-12 | 0.8    | 19590        | 660     | 1440    | 6040        | 7.51E+28 | 6.03E+28 | 8.32E+31 | <a href="http://www.ledas.ac.uk/data/2XMM/0398_0111410101_002/C0111410101EPX000SRCSUM0001.HTM">http://www.ledas.ac.uk/data/2XMM/0398_0111410101_002/C0111410101EPX000SRCSUM0001.HTM</a> |
| 40682 | 1       | 31822 | eps Eri                  | FALSE       | FALSE     | trend, fall   |       | 1.03E-11 |          |        |              |         |         |             | 1.28E+28 |          |          | <a href="http://www.ledas.ac.uk/data/2XMM/0570_0112880501_002/C0112880501EPX000SRCSUM0001.HTM">http://www.ledas.ac.uk/data/2XMM/0570_0112880501_002/C0112880501EPX000SRCSUM0001.HTM</a> |
| 42075 | 1       | 32605 | HR 1099                  | FALSE       | FALSE     | trend, fall   |       | 5.43E-11 |          |        |              |         |         |             | 6.11E+30 |          |          | <a href="http://www.ledas.ac.uk/data/2XMM/0221_0134540101_002/C0134540101EPX000SRCSUM0001.HTM">http://www.ledas.ac.uk/data/2XMM/0221_0134540101_002/C0134540101EPX000SRCSUM0001.HTM</a> |
| 42078 | 1       | 32605 | HR 1099                  | FALSE       | FALSE     | trend, rise   | 67.9  | 1.07E-10 | 1.79E-11 | 0.2    | 29600        | 4610    |         | 4610        | 1.20E+31 | 2.02E+30 | 8.02E+33 | <a href="http://www.ledas.ac.uk/data/2XMM/0132_0129350201_004/C0129350201EPX000SRCSUM0001.HTM">http://www.ledas.ac.uk/data/2XMM/0132_0129350201_004/C0129350201EPX000SRCSUM0001.HTM</a> |
| 42082 | 1       | 32605 | HR 1099                  | FALSE       | TRUE      | flare         | 124.9 | 1.10E-10 | 8.76E-11 | 0.8    | 50990        | 4320    | 3670    | 7990        | 1.24E+31 | 9.87E+30 | 6.41E+34 | <a href="http://www.ledas.ac.uk/data/2XMM/0036_0117890901_001/C0117890901EPX000SRCSUM0001.HTM">http://www.ledas.ac.uk/data/2XMM/0036_0117890901_001/C0117890901EPX000SRCSUM0001.HTM</a> |
| 42073 | 1       | 32605 | HR 1099                  | FALSE       | TRUE      | flare         | 43.3  | 7.06E-11 | 1.99E-11 | 0.3    | 14040        | 4400    | 7350    | 11750       | 7.95E+30 | 2.24E+30 | 1.31E+34 | <a href="http://www.ledas.ac.uk/data/2XMM/0310_0134540401_002/C0134540401EPX000SRCSUM0001.HTM">http://www.ledas.ac.uk/data/2XMM/0310_0134540401_002/C0134540401EPX000SRCSUM0001.HTM</a> |
| 42842 | 1       | 33211 | SDSS J033815.04+002926.0 | TRUE        | TRUE      | flare         | 12.8  | 5.28E-14 | 2.82E-12 | 53.4   | 12600        | 560     | 840     | 1400        | 3.18E+30 | 1.70E+32 | 1.52E+35 | <a href="http://www.ledas.ac.uk/data/2XMM/0404_0036540101_002/C0036540101EPX000SRCSUM0001.HTM">http://www.ledas.ac.uk/data/2XMM/0404_0036540101_002/C0036540101EPX000SRCSUM0001.HTM</a> |
| 44374 | 1       | 34580 | V471 Tau                 | TRUE        | TRUE      | flare         | 14.8  | 3.38E-12 | 2.78E-12 | 0.8    | 15290        | 380     | 3510    | 3890        | 7.84E+29 | 6.46E+29 | 1.28E+33 | <a href="http://www.ledas.ac.uk/data/2XMM/0851_0203260101_001/C0203260101EPX000SRCSUM0001.HTM">http://www.ledas.ac.uk/data/2XMM/0851_0203260101_001/C0203260101EPX000SRCSUM0001.HTM</a> |
| 45610 | 1       | 35718 | 2MASS J04072181-1210033  | TRUE        | TRUE      | flare         | 9.1   | 4.58E-13 | 1.06E-12 | 2.3    | 31710        | 980     | 1610    | 2590        | 8.57E+30 | 1.98E+31 | 3.11E+34 | <a href="http://www.ledas.ac.uk/data/2XMM/0944_0202210301_001/C0202210301EPX000SRCSUM0002.HTM">http://www.ledas.ac.uk/data/2XMM/0944_0202210301_001/C0202210301EPX000SRCSUM0002.HTM</a> |
| 45610 | 2       | 35718 | 2MASS J04072181-1210033  | TRUE        | TRUE      | flare         | 35.2  | 4.58E-13 | 3.39E-12 | 7.4    | 73430        | 2940    | 3920    | 6860        | 8.57E+30 | 6.35E+31 | 3.22E+35 | <a href="http://www.ledas.ac.uk/data/2XMM/0944_0202210301_001/C0202210301EPX000SRCSUM0002.HTM">http://www.ledas.ac.uk/data/2XMM/0944_0202210301_001/C0202210301EPX000SRCSUM0002.HTM</a> |
| 45611 | 1       | 35718 | 2MASS J04072181-1210033  | TRUE        | TRUE      | flare         | 15.3  | 3.20E-13 | 3.45E-13 | 1.1    | 20610        | 2970    | 3510    | 6480        | 6.00E+30 | 6.47E+30 | 2.85E+34 | <a href="http://www.ledas.ac.uk/data/2XMM/0945_0202210401_001/C0202210401EPX000SRCSUM0002.HTM">http://www.ledas.ac.uk/data/2XMM/0945_0202210401_001/C0202210401EPX000SRCSUM0002.HTM</a> |
| 45611 | 2       | 35718 | 2MASS J04072181-1210033  | TRUE        | TRUE      | flare         | 27.3  | 3.20E-13 | 4.20E-13 | 1.3    | 39150        | 2340    | 12420   | 14760       | 6.00E+30 | 7.87E+30 | 7.77E+34 | <a href="http://www.ledas.ac.uk/data/2XMM/0945_0202210401_001/C0202210401EPX000SRCSUM0002.HTM">http://www.ledas.ac.uk/data/2XMM/0945_0202210401_001/C0202210401EPX000SRCSUM0002.HTM</a> |
| 45611 | 3       | 35718 | 2MASS J04072181-1210033  | TRUE        | TRUE      | flare         | 16.9  | 3.20E-13 | 3.68E-13 | 1.1    | 60750        | 380     | 3870    | 5850        | 6.00E+30 | 6.89E+30 | 3.00E+34 | <a href="http://www.ledas.ac.uk/data/2XMM/0945_0202210401_001/C0202210401EPX000SRCSUM0002.HTM">http://www.ledas.ac.uk/data/2XMM/0945_0202210401_001/C0202210401EPX000SRCSUM0002.HTM</a> |
| 46637 | 1       | 36574 | V410 Tau                 | TRUE        | TRUE      | flare         | 50.0  | 1.93E-12 | 3.11E-12 | 1.6    | 58580        | 17260   | 9220    | 26480       | 2.23E+30 | 3.39E+30 | 5.29E+34 | <a href="http://www.ledas.ac.uk/data/2XMM/0230_0086360301_002/C0086360301EPX000SRCSUM0001.HTM">http://www.ledas.ac.uk/data/2XMM/0230_0086360301_002/C0086360301EPX000SRCSUM0001.HTM</a> |
| 46636 | 1       | 36574 | V410 Tau                 | TRUE        | TRUE      | flare         | 8.7   | 1.77E-12 | 7.00E-13 | 0.4    | 35080        | 960     | 1740    | 2700        | 2.05E+30 | 8.08E+29 | 1.16E+33 | <a href="http://www.ledas.ac.uk/data/2XMM/0230_0086360401_002/C0086360401EPX000SRCSUM0001.HTM">http://www.ledas.ac.uk/data/2XMM/0230_0086360401_002/C0086360401EPX000SRCSUM0001.HTM</a> |
| 47912 | 1       | 37582 | HD 283572                | TRUE        | FALSE     | gradual       | 37.1  | 4.41E-12 | 1.71E-12 | 0.4    | 16890        | 10700   | 5030    | 15730       | 8.62E+30 | 3.34E+30 | 3.44E+34 | <a href="http://www.ledas.ac.uk/data/2XMM/0136_0101440701_005/C0101440701EPX000SRCSUM0001.HTM">http://www.ledas.ac.uk/data/2XMM/0136_0101440701_005/C0101440701EPX000SRCSUM0001.HTM</a> |
| 47918 | 1       | 37588 | T Tau                    | FALSE       | FALSE     | trend, fall   |       | 1.82E-12 |          |        |              |         |         |             | 7.24E+30 |          |          | <a href="http://www.ledas.ac.uk/data/2XMM/1041_0301500101_002/C0301500101EPX000SRCSUM0001.HTM">http://www.ledas.ac.uk/data/2XMM/1041_0301500101_002/C0301500101EPX000SRCSUM0001.HTM</a> |
| 48185 | 1       | 37825 | VB 50                    | TRUE        | TRUE      | flare         | 50.5  | 2.69E-12 | 1.04E-11 | 3.9    | 36990        | 1080    | 3140    | 4220        | 6.20E+29 | 2.40E+30 | 6.23E+33 | <a href="http://www.ledas.ac.uk/data/2XMM/0138_0101440601_002/C0101440601EPX000SRCSUM0001.HTM">http://www.ledas.ac.uk/data/2XMM/0138_0101440601_002/C0101440601EPX000SRCSUM0001.HTM</a> |
| 48184 | 1       | 37825 | VB 50                    | TRUE        | TRUE      | flare         | 15.4  | 2.38E-12 | 1.25E-12 | 0.5    | 28680        | 380     | 1100    | 1480        | 5.50E+29 | 2.88E+29 | 3.45E+32 | <a href="http://www.ledas.ac.uk/data/2XMM/0410_0101441501_002/C0101441501EPX000SRCSUM0001.HTM">http://www.ledas.ac.uk/data/2XMM/0410_0101441501_002/C0101441501EPX000SRCSUM0001.HTM</a> |
| 48184 | 2       | 37825 | VB 50                    | TRUE        | TRUE      | flare         | 14.0  | 2.14E-12 | 9.99E-13 | 0.5    | 42180        | 620     | 2300    | 2920        | 4.95E+29 | 2.30E+29 | 3.96E+32 | <a href="http://www.ledas.ac.uk/data/2XMM/0410_0101441501_002/C0101441501EPX000SRCSUM0001.HTM">http://www.ledas.ac.uk/data/2XMM/0410_0101441501_002/C0101441501EPX000SRCSUM0001.HTM</a> |
| 48976 | 1       | 38388 | 78 Tau                   | TRUE        | TRUE      | flare         | 7.3   | 1.15E-13 | 3.36E-13 | 2.9    | 10350        | 900     | 450     | 900         | 2.94E+28 | 8.54E+28 | 7.07E+31 | <a href="http://www.ledas.ac.uk/data/2XMM/0135_0101440501_005/C0101440501EPX000SRCSUM0003.HTM">http://www.ledas.ac.uk/data/2XMM/0135_0101440501_005/C0101440501EPX000SRCSUM0003.HTM</a> |
| 48976 | 2       | 38388 | 78 Tau                   | TRUE        | TRUE      | flare         | 8.2   | 1.17E-13 | 1.04E-13 | 0.9    | 27000        | 3150    | 2250    | 5400        | 2.97E+28 | 2.64E+28 | 1.43E+32 | <a href="http://www.ledas.ac.uk/data/2XMM/0135_0101440501_005/C0101440501EPX000SRCSUM0003.HTM">http://www.ledas.ac.uk/data/2XMM/0135_0101440501_005/C0101440501EPX000SRCSUM0003.HTM</a> |
| 49620 | 1       | 38879 | HD 285845                | TRUE        | TRUE      | flare         | 18.1  | 1.58E-12 | 2.74E-12 | 1.7    | 1440         | 390     | 3330    | 3720        | 1.53E+30 | 2.65E+30 | 6.51E+33 | <a href="http://www.ledas.ac.uk/data/2XMM/0138_0109060301_004/C0109060301EPX000SRCSUM0001.HTM">http://www.ledas.ac.uk/data/2XMM/0138_0109060301_004/C0109060301EPX000SRCSUM0001.HTM</a> |
| 49620 | 2       | 38879 | HD 285845                | TRUE        | TRUE      | flare         | 21.0  | 1.58E-12 | 2.85E-12 | 1.6    | 8220         | 1290    | 2220    | 3510        | 1.53E+30 | 2.50E+30 | 7.89E+33 | <a href="http://www.ledas.ac.uk/data/2XMM/0138_0109060301_004/C0109060301EPX000SRCSUM0001.HTM">http://www.ledas.ac.uk/data/2XMM/0138_0109060301_004/C0109060301EPX000SRCSUM0001.HTM</a> |
| 49620 | 3       | 38879 | HD 285845                | TRUE        |           |               |       |          |          |        |              |         |         |             |          |          |          |                                                                                                                                                                                         |

| DETID  | EventNr | SRCD   | Star_Name               | ProfileFlag | FlareFlag | EventType     | SNR  | fx_quies | fx_peak  | r_peak | quies_t_peak | dt_rise | dt_fall | dt_duration | Lx_quies | Lx_peak  | Ex       | DSummaryLink                                                                                                                                                                              |
|--------|---------|--------|-------------------------|-------------|-----------|---------------|------|----------|----------|--------|--------------|---------|---------|-------------|----------|----------|----------|-------------------------------------------------------------------------------------------------------------------------------------------------------------------------------------------|
| 71057  | 1       | 54947  | chi01 Ori               | TRUE        | TRUE      | flare         | 5.6  | 9.01E-12 | 4.74E-12 | 0.5    | 23360        | 570     | 790     | 1360        | 8.09E+28 | 4.25E+28 | 1.75E+31 | <a href="http://www.ledas.ac.uk/data/2XMM/0243_0111500101_002/C0111500101EPX000SRCSUM0001.HTM">http://www.ledas.ac.uk/data/2XMM/0243_0111500101_002/C0111500101EPX000SRCSUM0001.HTM</a>   |
| 75409  | 1       | 58326  | SV Cam                  | TRUE        | TRUE      | flare         | 43.7 | 2.61E-12 | 2.48E-12 | 1.0    | 40840        | 2080    | 2540    | 4620        | 2.41E+30 | 2.30E+30 | 7.75E+33 | <a href="http://www.ledas.ac.uk/data/2XMM/0238_0029340101_003/C0029340101EPX000SRCSUM0001.HTM">http://www.ledas.ac.uk/data/2XMM/0238_0029340101_003/C0029340101EPX000SRCSUM0001.HTM</a>   |
| 75409  | 2       | 58326  | SV Cam                  | TRUE        | TRUE      | flare         | 55.4 | 2.61E-12 | 3.06E-12 | 1.2    | 46940        | 1290    | 5070    | 6360        | 2.41E+30 | 2.83E+30 | 1.14E+34 | <a href="http://www.ledas.ac.uk/data/2XMM/0238_0029340101_003/C0029340101EPX000SRCSUM0001.HTM">http://www.ledas.ac.uk/data/2XMM/0238_0029340101_003/C0029340101EPX000SRCSUM0001.HTM</a>   |
| 75410  | 1       | 58326  | SV Cam                  | TRUE        | TRUE      | flare         | 15.8 | 4.31E-12 | 2.53E-12 | 0.6    | 55000        | 2980    | 3280    | 6260        | 3.99E+30 | 2.34E+30 | 7.89E+33 | <a href="http://www.ledas.ac.uk/data/2XMM/0700_0029340201_002/C0029340201EPX000SRCSUM0001.HTM">http://www.ledas.ac.uk/data/2XMM/0700_0029340201_002/C0029340201EPX000SRCSUM0001.HTM</a>   |
| 79319  | 1       | 61056  | HD 51141                | TRUE        | TRUE      | flare         | 7.3  | 2.51E-14 | 3.31E-14 | 1.3    | 43750        | 2500    | 6250    | 8750        | 1.88E+28 | 2.47E+28 | 1.95E+32 | <a href="http://www.ledas.ac.uk/data/2XMM/0232_0022340201_002/C0022340201EPX000SRCSUM0009.HTM">http://www.ledas.ac.uk/data/2XMM/0232_0022340201_002/C0022340201EPX000SRCSUM0009.HTM</a>   |
| 80086  | 1       | 61727  | HD 59581                | TRUE        | TRUE      | flare         | 9.0  | 1.05E-12 | 1.47E-12 | 1.4    | 32400        | 2400    | 1950    | 4350        | 1.34E+30 | 1.87E+30 | 5.97E+33 | <a href="http://www.ledas.ac.uk/data/2XMM/0872_0164560901_002/C0164560901EPX000SRCSUM0003.HTM">http://www.ledas.ac.uk/data/2XMM/0872_0164560901_002/C0164560901EPX000SRCSUM0003.HTM</a>   |
| 81491  | 1       | 62784  | YZ CMi                  | TRUE        | TRUE      | flare         | 10.6 | 6.91E-12 | 5.55E-12 | 0.8    | 16040        | 590     | 330     | 920         | 2.93E+28 | 2.36E+28 | 1.16E+31 | <a href="http://www.ledas.ac.uk/data/2XMM/0153_0111460101_002/C0111460101EPX000SRCSUM0001.HTM">http://www.ledas.ac.uk/data/2XMM/0153_0111460101_002/C0111460101EPX000SRCSUM0001.HTM</a>   |
| 81491  | 2       | 62784  | YZ CMi                  | TRUE        | TRUE      | flare         | 16.5 | 6.91E-12 | 5.49E-12 | 0.8    | 21140        | 760     | 950     | 1710        | 2.93E+28 | 2.33E+28 | 2.54E+31 | <a href="http://www.ledas.ac.uk/data/2XMM/0153_0111460101_002/C0111460101EPX000SRCSUM0001.HTM">http://www.ledas.ac.uk/data/2XMM/0153_0111460101_002/C0111460101EPX000SRCSUM0001.HTM</a>   |
| 81491  | 3       | 62784  | YZ CMi                  | TRUE        | TRUE      | flare         | 20.6 | 6.91E-12 | 1.18E-11 | 1.7    | 24040        | 280     | 620     | 900         | 2.93E+28 | 4.99E+28 | 2.68E+31 | <a href="http://www.ledas.ac.uk/data/2XMM/0153_0111460101_002/C0111460101EPX000SRCSUM0001.HTM">http://www.ledas.ac.uk/data/2XMM/0153_0111460101_002/C0111460101EPX000SRCSUM0001.HTM</a>   |
| 89993  | 1       | 67988  | 2MASS J08322856+5245330 | TRUE        | TRUE      | flare         | 8.4  | 1.61E-14 | 1.29E-13 | 8.0    | 18720        | 4160    | 16640   | 20800       | 6.23E+26 | 5.00E+27 | 7.91E+31 | <a href="http://www.ledas.ac.uk/data/2XMM/0437_0092800201_003/C0092800201EPX000SRCSUM000F.HTM">http://www.ledas.ac.uk/data/2XMM/0437_0092800201_003/C0092800201EPX000SRCSUM000F.HTM</a>   |
| 91247  | 1       | 69047  | pi.01 UMa               | TRUE        | TRUE      | flare         | 23.0 | 3.16E-12 | 3.91E-12 | 1.2    | 25470        | 1540    | 2840    | 4380        | 7.80E+28 | 9.63E+28 | 2.57E+32 | <a href="http://www.ledas.ac.uk/data/2XMM/0166_0111400101_002/C0111400101EPX000SRCSUM0001.HTM">http://www.ledas.ac.uk/data/2XMM/0166_0111400101_002/C0111400101EPX000SRCSUM0001.HTM</a>   |
| 91247  | 2       | 69047  | pi.01 UMa               | TRUE        | TRUE      | flare         | 11.9 | 3.16E-12 | 3.93E-12 | 1.2    | 32170        | 570     | 1720    | 2290        | 7.80E+28 | 9.69E+28 | 8.88E+31 | <a href="http://www.ledas.ac.uk/data/2XMM/0166_0111400101_002/C0111400101EPX000SRCSUM0001.HTM">http://www.ledas.ac.uk/data/2XMM/0166_0111400101_002/C0111400101EPX000SRCSUM0001.HTM</a>   |
| 91420  | 1       | 69219  | HD 73709                | FALSE       | TRUE      | flare         | 6.8  | 6.83E-15 | 1.33E-13 | 19.5   |              |         | 11350   | 11350       | 2.64E+28 | 5.16E+29 | 3.81E+33 | <a href="http://www.ledas.ac.uk/data/2XMM/0168_0101440401_002/C0101440401EPX000SRCSUM0001A.HTM">http://www.ledas.ac.uk/data/2XMM/0168_0101440401_002/C0101440401EPX000SRCSUM0001A.HTM</a> |
| 93362  | 1       | 70721  | CD-45 4602              | TRUE        | FALSE     | indeterminate |      |          | 0        |        |              |         |         |             |          |          |          | <a href="http://www.ledas.ac.uk/data/2XMM/0718_0162360101_003/C0162360101EPX000SRCSUM0003.HTM">http://www.ledas.ac.uk/data/2XMM/0718_0162360101_003/C0162360101EPX000SRCSUM0003.HTM</a>   |
| 93359  | 1       | 70721  | CD-45 4602              | TRUE        | TRUE      | flare         | 8.7  | 1.11E-13 | 2.33E-13 | 2.1    | 23040        | 2880    | 3840    | 6720        | 6.88E+28 | 1.44E+29 | 6.89E+32 | <a href="http://www.ledas.ac.uk/data/2XMM/0252_0112870301_002/C0112870301EPX000SRCSUM0004.HTM">http://www.ledas.ac.uk/data/2XMM/0252_0112870301_002/C0112870301EPX000SRCSUM0004.HTM</a>   |
| 95682  | 1       | 72877  | XY UMa                  | TRUE        | TRUE      | flare         | 13.5 | 3.29E-12 | 1.28E-12 | 0.4    | 43940        | 830     | 2540    | 3370        | 1.73E+30 | 6.71E+29 | 1.16E+33 | <a href="http://www.ledas.ac.uk/data/2XMM/0971_0200960101_001/C0200960101EPX000SRCSUM0001.HTM">http://www.ledas.ac.uk/data/2XMM/0971_0200960101_001/C0200960101EPX000SRCSUM0001.HTM</a>   |
| 95682  | 2       | 72877  | XY UMa                  | TRUE        | TRUE      | flare         | 30.0 | 3.14E-12 | 1.73E-12 | 0.6    | 55740        | 2120    | 10460   | 12580       | 1.65E+30 | 9.07E+29 | 5.79E+33 | <a href="http://www.ledas.ac.uk/data/2XMM/0971_0200960101_001/C0200960101EPX000SRCSUM0001.HTM">http://www.ledas.ac.uk/data/2XMM/0971_0200960101_001/C0200960101EPX000SRCSUM0001.HTM</a>   |
| 95682  | 3       | 72877  | XY UMa                  | FALSE       | FALSE     | poor bgd sub? | 16.6 | 3.19E-12 | 2.86E-12 | 0.9    | 82390        | 2460    | 600     | 3060        | 1.67E+30 | 1.50E+30 | 1.80E+33 | <a href="http://www.ledas.ac.uk/data/2XMM/0971_0200960101_001/C0200960101EPX000SRCSUM0001.HTM">http://www.ledas.ac.uk/data/2XMM/0971_0200960101_001/C0200960101EPX000SRCSUM0001.HTM</a>   |
| 98763  | 1       | 75502  | LQ Hya                  | TRUE        | TRUE      | flare         | 25.2 | 1.44E-11 | 5.33E-12 | 0.4    | 24090        | 2600    | 2810    | 5410        | 5.97E+29 | 2.21E+29 | 1.03E+33 | <a href="http://www.ledas.ac.uk/data/2XMM/0625_0148880101_002/C0148880101EPX000SRCSUM0001.HTM">http://www.ledas.ac.uk/data/2XMM/0625_0148880101_002/C0148880101EPX000SRCSUM0001.HTM</a>   |
| 98764  | 1       | 75502  | LQ Hya                  | FALSE       | TRUE      | flare         | 16.0 | 1.53E-11 | 9.02E-12 | 0.6    | 190          | 130     | 1340    | 1470        | 6.36E+29 | 3.74E+29 | 3.61E+32 | <a href="http://www.ledas.ac.uk/data/2XMM/0724_0148880301_002/C0148880301EPX000SRCSUM0001.HTM">http://www.ledas.ac.uk/data/2XMM/0724_0148880301_002/C0148880301EPX000SRCSUM0001.HTM</a>   |
| 98764  | 2       | 75502  | LQ Hya                  | TRUE        | TRUE      | flare         | 13.5 | 1.53E-11 | 9.74E-12 | 0.6    | 12640        | 320     | 740     | 1060        | 6.36E+29 | 4.04E+29 | 2.58E+32 | <a href="http://www.ledas.ac.uk/data/2XMM/0724_0148880301_002/C0148880301EPX000SRCSUM0001.HTM">http://www.ledas.ac.uk/data/2XMM/0724_0148880301_002/C0148880301EPX000SRCSUM0001.HTM</a>   |
| 99591  | 1       | 76251  | HD 83698                | TRUE        | TRUE      | flare         | 8.1  | 3.61E-14 | 8.58E-14 | 2.4    | 43520        | 2720    | 2040    | 4760        | 1.13E+31 | 2.70E+28 | 8.60E+31 | <a href="http://www.ledas.ac.uk/data/2XMM/0813_0203270101_001/C0203270101EPX000SRCSUM0002.HTM">http://www.ledas.ac.uk/data/2XMM/0813_0203270101_001/C0203270101EPX000SRCSUM0002.HTM</a>   |
| 101535 | 1       | 77959  | 2MASS J09553615+6954487 | TRUE        | FALSE     | indeterminate |      | 2.11E-13 |          |        |              |         |         |             |          |          |          | <a href="http://www.ledas.ac.uk/data/2XMM/0800_0206080101_001/C0206080101EPX000SRCSUM0001.HTM">http://www.ledas.ac.uk/data/2XMM/0800_0206080101_001/C0206080101EPX000SRCSUM0001.HTM</a>   |
| 108025 | 1       | 82640  | AD Leo                  | FALSE       | TRUE      | flare         | 43.8 | 1.60E-11 | 2.22E-11 | 1.4    | 490          | 310     | 5360    | 5670        | 4.56E+28 | 6.34E+28 | 1.37E+32 | <a href="http://www.ledas.ac.uk/data/2XMM/0262_0111440101_002/C0111440101EPX000SRCSUM0001.HTM">http://www.ledas.ac.uk/data/2XMM/0262_0111440101_002/C0111440101EPX000SRCSUM0001.HTM</a>   |
| 108025 | 2       | 82640  | AD Leo                  | TRUE        | TRUE      | flare         | 23.6 | 1.34E-11 | 8.12E-12 | 0.6    | 15090        | 1350    | 2100    | 3450        | 3.83E+28 | 2.32E+28 | 5.04E+31 | <a href="http://www.ledas.ac.uk/data/2XMM/0262_0111440101_002/C0111440101EPX000SRCSUM0001.HTM">http://www.ledas.ac.uk/data/2XMM/0262_0111440101_002/C0111440101EPX000SRCSUM0001.HTM</a>   |
| 108025 | 3       | 82640  | AD Leo                  | TRUE        | TRUE      | flare         | 10.3 | 1.34E-11 | 4.90E-12 | 0.4    | 25890        | 740     | 930     | 1670        | 3.83E+28 | 1.40E+28 | 1.44E+31 | <a href="http://www.ledas.ac.uk/data/2XMM/0262_0111440101_002/C0111440101EPX000SRCSUM0001.HTM">http://www.ledas.ac.uk/data/2XMM/0262_0111440101_002/C0111440101EPX000SRCSUM0001.HTM</a>   |
| 108025 | 4       | 82640  | AD Leo                  | TRUE        | TRUE      | flare         | 12.1 | 1.34E-11 | 7.21E-12 | 0.5    | 29090        | 1040    | 1130    | 2170        | 3.83E+28 | 2.06E+28 | 1.92E+31 | <a href="http://www.ledas.ac.uk/data/2XMM/0262_0111440101_002/C0111440101EPX000SRCSUM0001.HTM">http://www.ledas.ac.uk/data/2XMM/0262_0111440101_002/C0111440101EPX000SRCSUM0001.HTM</a>   |
| 108025 | 5       | 82640  | AD Leo                  | TRUE        | TRUE      | flare         | 11.4 | 1.34E-11 | 4.86E-12 | 0.4    | 34190        | 2060    | 990     | 3050        | 3.83E+28 | 1.39E+28 | 2.10E+31 | <a href="http://www.ledas.ac.uk/data/2XMM/0262_0111440101_002/C0111440101EPX000SRCSUM0001.HTM">http://www.ledas.ac.uk/data/2XMM/0262_0111440101_002/C0111440101EPX000SRCSUM0001.HTM</a>   |
| 118876 | 1       | 89750  | NU UMa                  | TRUE        | TRUE      | flare         | 7.0  | 2.09E-13 | 5.19E-13 | 2.5    | 29640        | 780     | 2340    | 3120        | 2.79E+29 | 6.94E+29 | 1.94E+33 | <a href="http://www.ledas.ac.uk/data/2XMM/0544_0147511601_002/C0147511601EPX000SRCSUM0005.HTM">http://www.ledas.ac.uk/data/2XMM/0544_0147511601_002/C0147511601EPX000SRCSUM0005.HTM</a>   |
| 120401 | 1       | 90546  | CR Cha                  | TRUE        | TRUE      | flare         | 14.2 | 5.07E-13 | 4.19E-13 | 0.8    | 25410        | 3080    | 2800    | 5880        | 1.70E+30 | 1.41E+30 | 5.19E+33 | <a href="http://www.ledas.ac.uk/data/2XMM/0222_0067140201_002/C0067140201EPX000SRCSUM0001.HTM">http://www.ledas.ac.uk/data/2XMM/0222_0067140201_002/C0067140201EPX000SRCSUM0001.HTM</a>   |
| 121057 | 1       | 91087  | HD 95735                | TRUE        | TRUE      | flare         | 27.3 | 1.86E-12 | 1.85E-12 | 1.0    | 25440        | 400     | 1740    | 2140        | 1.45E+27 | 1.44E+27 | 1.94E+30 | <a href="http://www.ledas.ac.uk/data/2XMM/0810_0205370101_002/C0205370101EPX000SRCSUM0001.HTM">http://www.ledas.ac.uk/data/2XMM/0810_0205370101_002/C0205370101EPX000SRCSUM0001.HTM</a>   |
| 121057 | 2       | 91087  | HD 95735                | TRUE        | TRUE      | flare         | 47.1 | 1.86E-12 | 2.05E-12 | 1.1    | 31940        | 1560    | 3600    | 5160        | 1.45E+27 | 1.59E+27 | 5.34E+30 | <a href="http://www.ledas.ac.uk/data/2XMM/0810_0205370101_002/C0205370101EPX000SRCSUM0001.HTM">http://www.ledas.ac.uk/data/2XMM/0810_0205370101_002/C0205370101EPX000SRCSUM0001.HTM</a>   |
| 123749 | 1       | 92587  | GSC 09414-00787         | FALSE       | FALSE     | trend, rise   | 20.0 | 1.17E-12 | 1.55E-12 | 1.3    | 28600        | 6710    | 1540    | 8250        | 3.59E+30 | 4.75E+30 | 2.66E+34 | <a href="http://www.ledas.ac.uk/data/2XMM/0773_0203810201_002/C0203810201EPX000SRCSUM0001.HTM">http://www.ledas.ac.uk/data/2XMM/0773_0203810201_002/C0203810201EPX000SRCSUM0001.HTM</a>   |
| 130963 | 1       | 99128  | HD 104021               | FALSE       | FALSE     | gradual       | 63.1 | 2.38E-12 | 3.51E-12 | 1.5    | 24980        | 6240    | 12920   | 19160       | 3.58E+30 | 5.28E+30 | 7.86E+34 | <a href="http://www.ledas.ac.uk/data/2XMM/1111_0301430101_001/C0301430101EPX000SRCSUM0001.HTM">http://www.ledas.ac.uk/data/2XMM/1111_0301430101_001/C0301430101EPX000SRCSUM0001.HTM</a>   |
| 142357 | 1       | 107354 | HD 108984               | FALSE       | TRUE      | flare         | 7.9  | 5.61E-14 | 3.89E-13 | 6.9    |              |         | 2100    | 2100        | 4.47E+27 | 3.10E+28 | 7.46E+31 | <a href="http://www.ledas.ac.uk/data/2XMM/1022_0301450201_002/C0301450201EPX000SRCSUM0002.HTM">http://www.ledas.ac.uk/data/2XMM/1022_0301450201_002/C0301450201EPX000SRCSUM0002.HTM</a>   |
| 148010 | 1       | 112107 | IM Vir                  | TRUE        | TRUE      | flare         | 17.8 | 2.18E-12 | 1.83E-12 | 0.8    | 6690         | 930     | 1470    | 2400        | 2.10E+30 | 1.77E+30 | 3.02E+33 | <a href="http://www.ledas.ac.uk/data/2XMM/0842_0203270301_001/C0203270301EPX000SRCSUM0001.HTM">http://www.ledas.ac.uk/data/2XMM/0842_0203270301_001/C0203270301EPX000SRCSUM0001.HTM</a>   |
| 148010 | 2       | 112107 | IM Vir                  | TRUE        | TRUE      | flare         | 32.0 | 2.18E-12 | 2.46E-12 | 1.1    | 11220        | 1740    | 3720    | 5460        | 2.10E+30 | 2.37E+30 | 8.44E+33 | <a href="http://www.ledas.ac.uk/data/2XMM/0842_0203270301_001/C0203270301EPX000SRCSUM0001.HTM">http://www.ledas.ac.uk/data/2XMM/0842_0203270301_001/C0203270301EPX000SRCSUM0001.HTM</a>   |
| 148011 | 1       | 112107 | IM Vir                  | TRUE        | TRUE      | flare         | 6.4  | 2.51E-12 | 5.72E-12 | 0.2    | 11820        | 750     | 1140    | 1890        | 2.42E+30 | 5.51E+29 | 8.41E+32 | <a href="http://www.ledas.ac.uk/data/2XMM/0291_0060370201_002/C0060370201EPX000SRCSUM0001.HTM">http://www.ledas.ac.uk/data/2XMM/0291_0060370201_002/C0060370201EPX000SRCSUM0001.HTM</a>   |
| 148011 | 2       | 112107 | IM Vir                  | TRUE        | TRUE      | flare         | 9.8  | 2.14E-12 | 5.54E-13 | 0.3    | 24870        | 1200    | 2520    | 3720        | 2.06E+30 | 5.19E+29 | 1.71E+33 | <a href="http://www.ledas.ac.uk/data/2XMM/0291_0060370201_002/C0060370201EPX000SRCSUM0001.HTM">http://www.ledas.ac.uk/data/2XMM/0291_0060370201_002/C0060370201EPX000SRCSUM0001.HTM</a>   |
| 156921 | 1       | 119315 | 2MASS J13141103-1620235 | TRUE        | TRUE      | flare         | 6.2  | 8.89E-14 | 3.73E-13 | 4.2    | 45000        | 900     | 900     | 1800        | 2.83E+30 | 1.34E+31 | 1.80E+34 | <a href="http://www.ledas.ac.uk/data/2XMM/1113_0301290101_001/C0301290101EPX000SRCSUM0004.HTM">http://www.ledas.ac.uk/data/2XMM/1113_0301290101_001/C0301290101EPX000SRCSUM0004.HTM</a>   |
| 160700 | 1       | 122713 |                         |             |           |               |      |          |          |        |              |         |         |             |          |          |          |                                                                                                                                                                                           |

| DETID  | EventNr | SRCID  | Star_Name             | ProfileFlag | FlareFlag | EventType     | SNR  | fx_quies | fx_peak  | r_peak | quies | t_peak | dt_rise | dt_fall | dt_duration | Lx_quies | Lx_peak  | Ex       | DPsummaryLink                                                                                                                                                                           |
|--------|---------|--------|-----------------------|-------------|-----------|---------------|------|----------|----------|--------|-------|--------|---------|---------|-------------|----------|----------|----------|-----------------------------------------------------------------------------------------------------------------------------------------------------------------------------------------|
| 226652 | 1       | 174581 | VW Cep                | TRUE        | FALSE     | trend, fall   |      | 6.85E-12 |          |        |       |        |         |         |             | 6.24E+29 |          |          | <a href="http://www.ledas.ac.uk/data/2XMM/0529_0100650301_003/C0100650301EPX000SRCSUM0001.HTM">http://www.ledas.ac.uk/data/2XMM/0529_0100650301_003/C0100650301EPX000SRCSUM0001.HTM</a> |
| 226653 | 1       | 174581 | VW Cep                | TRUE        | FALSE     | indeterminate |      | 7.58E-12 |          |        |       |        |         |         |             | 6.90E+29 |          |          | <a href="http://www.ledas.ac.uk/data/2XMM/0515_0100650201_002/C0100650201EPX000SRCSUM0001.HTM">http://www.ledas.ac.uk/data/2XMM/0515_0100650201_002/C0100650201EPX000SRCSUM0001.HTM</a> |
| 226922 | 1       | 174842 | AT Mic                | TRUE        | TRUE      | flare         | 48.3 | 1.78E-11 | 1.53E-11 |        | 0.9   | 16390  | 640     | 3300    | 3940        | 2.44E+29 | 2.09E+29 | 6.32E+32 | <a href="http://www.ledas.ac.uk/data/2XMM/0156_0111510101_003/C0111510101EPX000SRCSUM0001.HTM">http://www.ledas.ac.uk/data/2XMM/0156_0111510101_003/C0111510101EPX000SRCSUM0001.HTM</a> |
| 227252 | 1       | 175166 | AU Mic                | TRUE        | TRUE      | flare         | 9.6  | 2.32E-11 | 8.05E-12 |        | 0.3   | 4790   | 600     | 1070    | 1670        | 2.72E+29 | 9.46E+28 | 7.27E+31 | <a href="http://www.ledas.ac.uk/data/2XMM/0155_0111420101_003/C0111420101EPX000SRCSUM0001.HTM">http://www.ledas.ac.uk/data/2XMM/0155_0111420101_003/C0111420101EPX000SRCSUM0001.HTM</a> |
| 227252 | 2       | 175166 | AU Mic                | TRUE        | TRUE      | flare         | 12.6 | 2.32E-11 | 6.49E-12 |        | 0.3   | 8340   | 1160    | 1440    | 2600        | 2.72E+29 | 7.63E+28 | 1.20E+32 | <a href="http://www.ledas.ac.uk/data/2XMM/0155_0111420101_003/C0111420101EPX000SRCSUM0001.HTM">http://www.ledas.ac.uk/data/2XMM/0155_0111420101_003/C0111420101EPX000SRCSUM0001.HTM</a> |
| 227252 | 3       | 175166 | AU Mic                | TRUE        | TRUE      | flare         | 17.1 | 2.07E-11 | 4.67E-12 |        | 0.2   | 22390  | 1410    | 2010    | 3420        | 2.43E+29 | 5.48E+28 | 1.80E+32 | <a href="http://www.ledas.ac.uk/data/2XMM/0155_0111420101_003/C0111420101EPX000SRCSUM0001.HTM">http://www.ledas.ac.uk/data/2XMM/0155_0111420101_003/C0111420101EPX000SRCSUM0001.HTM</a> |
| 227252 | 4       | 175166 | AU Mic                | TRUE        | TRUE      | flare         | 18.0 | 1.96E-11 | 1.28E-11 |        | 0.7   | 31570  | 290     | 1050    | 1340        | 2.30E+29 | 1.50E+29 | 1.24E+32 | <a href="http://www.ledas.ac.uk/data/2XMM/0155_0111420101_003/C0111420101EPX000SRCSUM0001.HTM">http://www.ledas.ac.uk/data/2XMM/0155_0111420101_003/C0111420101EPX000SRCSUM0001.HTM</a> |
| 227252 | 5       | 175166 | AU Mic                | TRUE        | TRUE      | flare         | 15.2 | 1.86E-11 | 8.54E-12 |        | 0.5   | 49930  | 780     | 830     | 1610        | 2.18E+29 | 1.00E+29 | 1.08E+32 | <a href="http://www.ledas.ac.uk/data/2XMM/0155_0111420101_003/C0111420101EPX000SRCSUM0001.HTM">http://www.ledas.ac.uk/data/2XMM/0155_0111420101_003/C0111420101EPX000SRCSUM0001.HTM</a> |
| 227252 | 6       | 175166 | AU Mic                | TRUE        | TRUE      | flare         | 29.9 | 1.86E-11 | 1.57E-11 |        | 0.8   | 53590  | 1440    | 1060    | 2500        | 2.18E+29 | 1.85E+29 | 2.86E+32 | <a href="http://www.ledas.ac.uk/data/2XMM/0155_0111420101_003/C0111420101EPX000SRCSUM0001.HTM">http://www.ledas.ac.uk/data/2XMM/0155_0111420101_003/C0111420101EPX000SRCSUM0001.HTM</a> |
| 229724 | 1       | 177371 | 61 Cyg A              | TRUE        | TRUE      | flare         | 24.1 | 1.34E-12 | 3.87E-12 |        | 2.9   | 3360   | 140     | 880     | 1020        | 1.94E+27 | 5.63E+27 | 3.67E+30 | <a href="http://www.ledas.ac.uk/data/2XMM/0724_0041741001_002/C0041741001EPX000SRCSUM0001.HTM">http://www.ledas.ac.uk/data/2XMM/0724_0041741001_002/C0041741001EPX000SRCSUM0001.HTM</a> |
| 229734 | 1       | 177375 | 61 Cyg B              | TRUE        | FALSE     | indeterminate |      | 3.93E-13 |          |        |       |        |         |         |             | 5.74E+26 |          |          | <a href="http://www.ledas.ac.uk/data/2XMM/0805_0041741101_002/C0041741101EPX000SRCSUM0002.HTM">http://www.ledas.ac.uk/data/2XMM/0805_0041741101_002/C0041741101EPX000SRCSUM0002.HTM</a> |
| 229736 | 1       | 177375 | 61 Cyg B              | TRUE        | TRUE      | flare         | 56.8 | 6.21E-13 | 1.08E-11 |        | 17.4  | 6790   | 730     | 4500    | 5230        | 9.08E+26 | 1.58E+28 | 4.89E+31 | <a href="http://www.ledas.ac.uk/data/2XMM/0898_0143630101_001/C0143630101EPX000SRCSUM0001.HTM">http://www.ledas.ac.uk/data/2XMM/0898_0143630101_001/C0143630101EPX000SRCSUM0001.HTM</a> |
| 231002 | 1       | 178313 | SAO 10050             | TRUE        | TRUE      | flare         | 10.9 | 7.54E-14 | 5.79E-13 |        | 7.7   | 31800  | 3600    | 7200    | 10800       | 4.80E+28 | 3.69E+29 | 3.17E+33 | <a href="http://www.ledas.ac.uk/data/2XMM/1036_0300490501_001/C0300490501EPX000SRCSUM0002.HTM">http://www.ledas.ac.uk/data/2XMM/1036_0300490501_001/C0300490501EPX000SRCSUM0002.HTM</a> |
| 239075 | 1       | 185001 | EV Lac                | TRUE        | TRUE      | flare         | 18.4 | 1.27E-11 | 6.10E-12 |        | 0.5   | 2490   | 1590    | 1560    | 3150        | 4.00E+28 | 1.92E+28 | 3.61E+31 | <a href="http://www.ledas.ac.uk/data/2XMM/0272_0111450101_002/C0111450101EPX000SRCSUM0001.HTM">http://www.ledas.ac.uk/data/2XMM/0272_0111450101_002/C0111450101EPX000SRCSUM0001.HTM</a> |
| 239075 | 2       | 185001 | EV Lac                | TRUE        | TRUE      | flare         | 12.5 | 1.29E-11 | 6.29E-12 |        | 0.5   | 9590   | 790     | 270     | 1060        | 4.04E+28 | 1.97E+28 | 1.45E+31 | <a href="http://www.ledas.ac.uk/data/2XMM/0272_0111450101_002/C0111450101EPX000SRCSUM0001.HTM">http://www.ledas.ac.uk/data/2XMM/0272_0111450101_002/C0111450101EPX000SRCSUM0001.HTM</a> |
| 239075 | 3       | 185001 | EV Lac                | TRUE        | TRUE      | flare         | 22.0 | 1.29E-11 | 8.36E-12 |        | 0.6   | 12140  | 900     | 1090    | 1990        | 4.04E+28 | 2.62E+28 | 3.73E+31 | <a href="http://www.ledas.ac.uk/data/2XMM/0272_0111450101_002/C0111450101EPX000SRCSUM0001.HTM">http://www.ledas.ac.uk/data/2XMM/0272_0111450101_002/C0111450101EPX000SRCSUM0001.HTM</a> |
| 239075 | 4       | 185001 | EV Lac                | TRUE        | TRUE      | flare         | 7.0  | 1.29E-11 | 3.84E-12 |        | 0.3   | 16740  | 370     | 910     | 1280        | 4.04E+28 | 1.20E+28 | 8.37E+30 | <a href="http://www.ledas.ac.uk/data/2XMM/0272_0111450101_002/C0111450101EPX000SRCSUM0001.HTM">http://www.ledas.ac.uk/data/2XMM/0272_0111450101_002/C0111450101EPX000SRCSUM0001.HTM</a> |
| 239075 | 5       | 185001 | EV Lac                | TRUE        | TRUE      | flare         | 30.6 | 1.29E-11 | 1.25E-11 |        | 1.0   | 21340  | 890     | 930     | 1820        | 4.04E+28 | 3.92E+28 | 5.25E+31 | <a href="http://www.ledas.ac.uk/data/2XMM/0272_0111450101_002/C0111450101EPX000SRCSUM0001.HTM">http://www.ledas.ac.uk/data/2XMM/0272_0111450101_002/C0111450101EPX000SRCSUM0001.HTM</a> |
| 239075 | 6       | 185001 | EV Lac                | TRUE        | TRUE      | flare         | 25.0 | 1.29E-11 | 1.13E-11 |        | 0.9   | 23790  | 650     | 610     | 1260        | 4.04E+28 | 3.53E+28 | 3.52E+31 | <a href="http://www.ledas.ac.uk/data/2XMM/0272_0111450101_002/C0111450101EPX000SRCSUM0001.HTM">http://www.ledas.ac.uk/data/2XMM/0272_0111450101_002/C0111450101EPX000SRCSUM0001.HTM</a> |
| 241508 | 1       | 187121 | HK Aqr                | TRUE        | TRUE      | flare         | 11.0 | 1.62E-12 | 1.22E-12 |        | 0.8   | 42740  | 940     | 2440    | 3380        | 9.61E+28 | 7.26E+28 | 1.59E+32 | <a href="http://www.ledas.ac.uk/data/2XMM/0996_0202360101_001/C0202360101EPX000SRCSUM0001.HTM">http://www.ledas.ac.uk/data/2XMM/0996_0202360101_001/C0202360101EPX000SRCSUM0001.HTM</a> |
| 241508 | 2       | 187121 | HK Aqr                | TRUE        | TRUE      | flare         | 8.3  | 1.62E-12 | 1.54E-12 |        | 0.9   | 48860  | 1380    | 2320    | 3700        | 9.61E+28 | 9.13E+28 | 1.19E+32 | <a href="http://www.ledas.ac.uk/data/2XMM/0996_0202360101_001/C0202360101EPX000SRCSUM0001.HTM">http://www.ledas.ac.uk/data/2XMM/0996_0202360101_001/C0202360101EPX000SRCSUM0001.HTM</a> |
| 241508 | 3       | 187121 | HK Aqr                | TRUE        | TRUE      | flare         | 8.5  | 1.54E-12 | 1.78E-12 |        | 1.2   | 74880  | 1360    | 620     | 1980        | 9.16E+28 | 1.06E+29 | 9.22E+31 | <a href="http://www.ledas.ac.uk/data/2XMM/0996_0202360101_001/C0202360101EPX000SRCSUM0001.HTM">http://www.ledas.ac.uk/data/2XMM/0996_0202360101_001/C0202360101EPX000SRCSUM0001.HTM</a> |
| 241508 | 4       | 187121 | HK Aqr                | FALSE       | FALSE     | poor bgd sub? | 29.1 | 1.42E-12 | 5.45E-12 |        | 3.8   | 101060 | 660     | 2320    | 2980        | 8.46E+28 | 3.23E+29 | 5.76E+32 | <a href="http://www.ledas.ac.uk/data/2XMM/0996_0202360101_001/C0202360101EPX000SRCSUM0001.HTM">http://www.ledas.ac.uk/data/2XMM/0996_0202360101_001/C0202360101EPX000SRCSUM0001.HTM</a> |
| 242179 | 1       | 187670 | 1RXS J231628.7+790531 | TRUE        | TRUE      | flare         | 78.7 | 1.35E-12 | 3.81E-11 |        | 28.3  | 14580  | 1660    | 5860    | 7520        | 4.87E+29 | 1.38E+31 | 7.01E+34 | <a href="http://www.ledas.ac.uk/data/2XMM/0742_0203060101_003/C0203060101EPX000SRCSUM0002.HTM">http://www.ledas.ac.uk/data/2XMM/0742_0203060101_003/C0203060101EPX000SRCSUM0002.HTM</a> |
| 242641 | 1       | 188039 | V368 Cep              | FALSE       | TRUE      | flare         | 22.1 | 1.61E-11 | 1.54E-11 |        | 1.0   | 40     | 40      | 1480    | 1520        | 7.11E+29 | 6.78E+29 | 5.80E+32 | <a href="http://www.ledas.ac.uk/data/2XMM/0742_0203060101_003/C0203060101EPX000SRCSUM0001.HTM">http://www.ledas.ac.uk/data/2XMM/0742_0203060101_003/C0203060101EPX000SRCSUM0001.HTM</a> |
| 242641 | 2       | 188039 | V368 Cep              | TRUE        | TRUE      | flare         | 23.4 | 1.61E-11 | 1.23E-11 |        | 0.8   | 20690  | 530     | 840     | 1370        | 7.11E+29 | 5.41E+29 | 5.97E+32 | <a href="http://www.ledas.ac.uk/data/2XMM/0742_0203060101_003/C0203060101EPX000SRCSUM0001.HTM">http://www.ledas.ac.uk/data/2XMM/0742_0203060101_003/C0203060101EPX000SRCSUM0001.HTM</a> |
| 242641 | 3       | 188039 | V368 Cep              | TRUE        | TRUE      | flare         | 16.5 | 1.61E-11 | 1.28E-11 |        | 0.8   | 22890  | 400     | 380     | 780         | 7.11E+29 | 5.63E+29 | 3.13E+32 | <a href="http://www.ledas.ac.uk/data/2XMM/0742_0203060101_003/C0203060101EPX000SRCSUM0001.HTM">http://www.ledas.ac.uk/data/2XMM/0742_0203060101_003/C0203060101EPX000SRCSUM0001.HTM</a> |
| 243984 | 1       | 189152 | EQ Peg                | TRUE        | FALSE     | gradual       | 40.7 | 1.23E-11 | 5.66E-12 |        | 0.5   | 11140  | 4550    | 2200    | 6750        | 5.61E+28 | 2.59E+28 | 9.65E+31 | <a href="http://www.ledas.ac.uk/data/2XMM/0107_0112880301_004/C0112880301EPX000SRCSUM0001.HTM">http://www.ledas.ac.uk/data/2XMM/0107_0112880301_004/C0112880301EPX000SRCSUM0001.HTM</a> |
| 243985 | 1       | 189152 | EQ Peg                | FALSE       | TRUE      | flare         | 21.9 | 1.27E-11 | 4.79E-12 |        | 0.4   | 2090   | 480     | 1800    | 2280        | 5.80E+28 | 2.19E+28 | 3.77E+31 | <a href="http://www.ledas.ac.uk/data/2XMM/0559_0147580301_002/C0147580301EPX000SRCSUM0001.HTM">http://www.ledas.ac.uk/data/2XMM/0559_0147580301_002/C0147580301EPX000SRCSUM0001.HTM</a> |
| 244744 | 1       | 189774 | Iam And               | TRUE        | FALSE     | trend, rise   |      | 5.41E-11 |          |        |       |        |         |         |             | 4.51E+30 |          |          | <a href="http://www.ledas.ac.uk/data/2XMM/0208_0099320101_002/C0099320101EPX000SRCSUM0001.HTM">http://www.ledas.ac.uk/data/2XMM/0208_0099320101_002/C0099320101EPX000SRCSUM0001.HTM</a> |

| Column Name   | Description                                                                                                    | Units       | Origin       |
|---------------|----------------------------------------------------------------------------------------------------------------|-------------|--------------|
| DETID         | a consecutive number which identifies each entry (detection) in the 2XMM catalogue                             |             | 2XMM         |
| EventNr       | a consecutive number which identifies each event in a light-curve                                              |             | this work    |
| SRCID         | a unique number assigned to a group of 2XMM catalogue entries (DETIDs) which are assumed to be the same source |             | 2XMM         |
| Star_Name     | identifying name for the star                                                                                  |             | SIMBAD+      |
| ProfileFlag   | = TRUE if event profile considered to be fully observed                                                        |             | this work    |
| FlareFlag     | = TRUE if event is considered to be a flare                                                                    |             | this work    |
| EventType     | event type: flare, trend, gradual, indeterminate, or periodic; see Sect. 3.1                                   |             | this work    |
| SNR           | signal:noise ratio of event, over timespan "duration"                                                          |             | this work    |
| fx_quies      | quiescent level, mean X-ray flux (total band, 0.2-12 keV)                                                      | erg/cm**2/s | this work    |
| fx_peak       | flare peak X-ray flux, above quiescent (total band, 0.2-12 keV)                                                | erg/cm**2/s | this work    |
| r_peak_quies  | flare peak:quiescent ratio, X-ray flux or luminosity                                                           |             | this work    |
| t_peak        | time of flare peak (relative to observation start)                                                             | s           | this work    |
| dt_rise       | flare rise time, 1/e to peak                                                                                   | s           | this work    |
| dt_fall       | flare fall time, peak to 1/e                                                                                   | s           | this work    |
| dt_duration   | flare duration, time between 1/e points                                                                        | s           | this work    |
| Lx_quies      | quiescent level, mean X-ray luminosity (total band, 0.2-12 keV)                                                | erg/s       | this work    |
| Lx_peak       | flare peak X-ray luminosity, above quiescent (total band, 0.2-12 keV)                                          | erg/s       | this work    |
| Ex            | flare X-ray emitted energy, within timespan "duration"                                                         | erg         | this work    |
| DPsummaryLink | URL link to 2XMM summary-results web page at LEDAS                                                             |             | 2XMM derived |

#### NOTES:

Description: for parameters from 2XMM & Tycho-2, more information may be found in those catalogues

Origin: 2XMM = values taken directly from 2XMM catalogue  
2XMM derived = based on values in 2XMM catalogue  
SIMBAD+ = taken from CDS SIMBAD database and other sources
