# Supplementary material for: A survey of stellar X-ray flares from the XMM-Newton serendipitous source catalogue: Hipparcos-Tycho cool stars
Source: arXiv:1506.05289 ancillary file (2015-06-17)

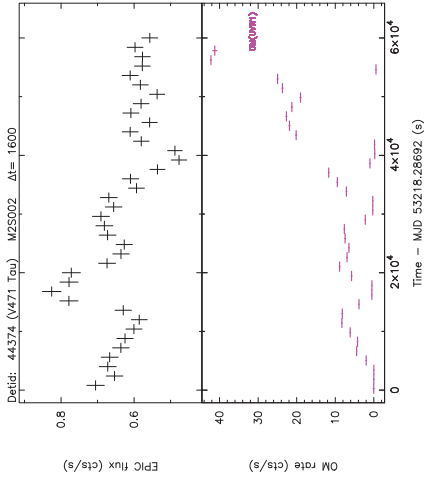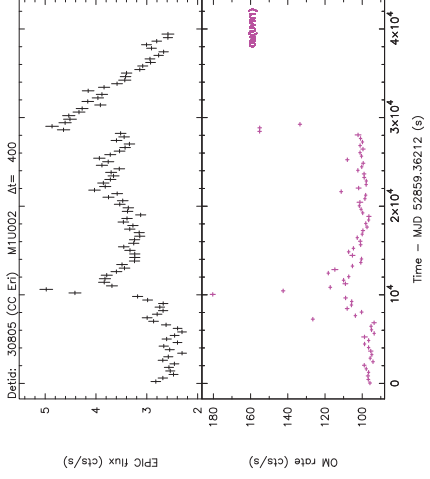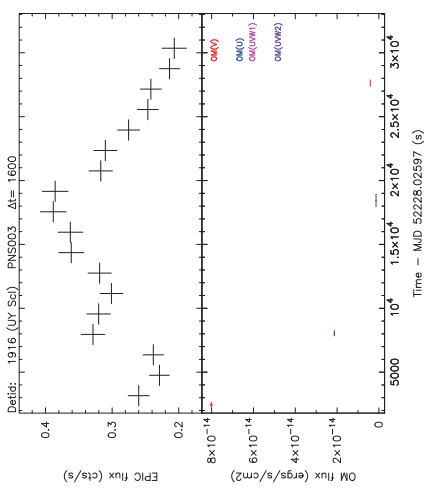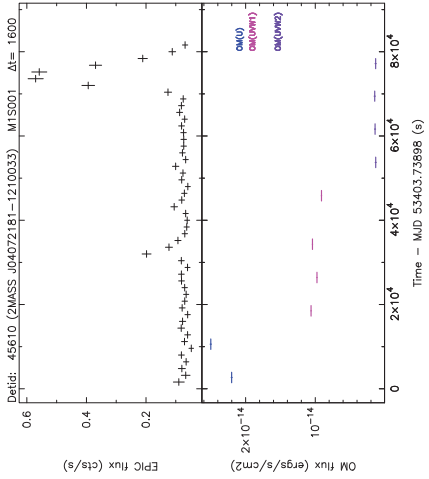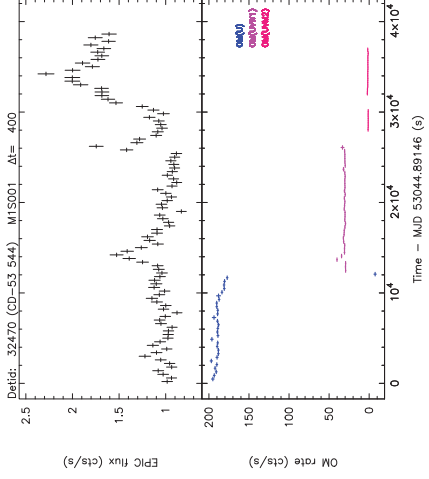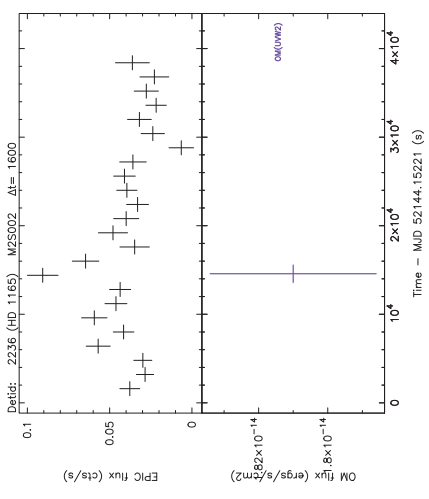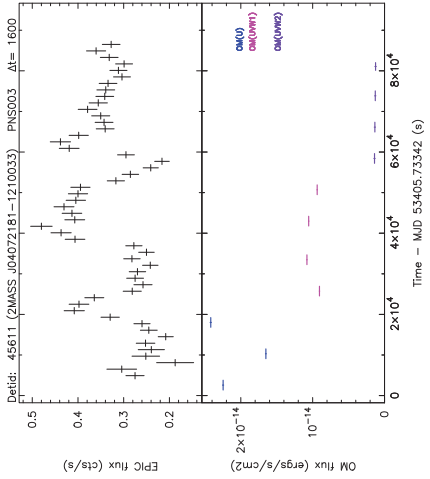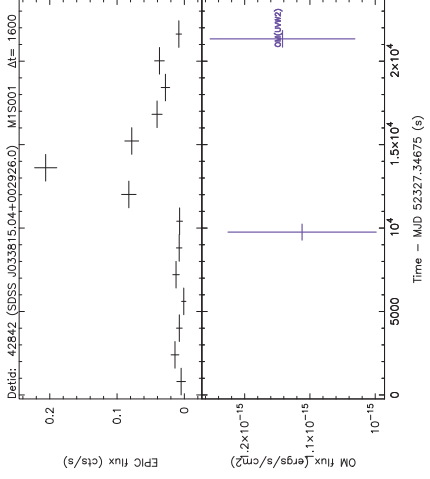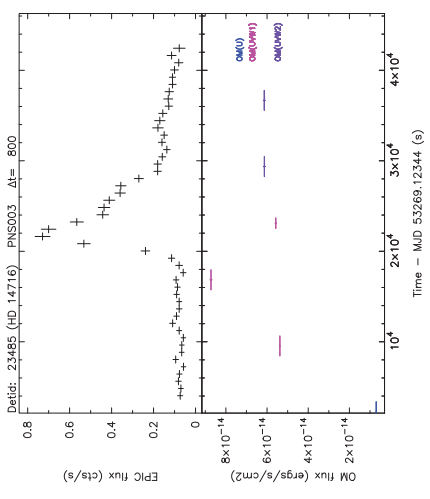

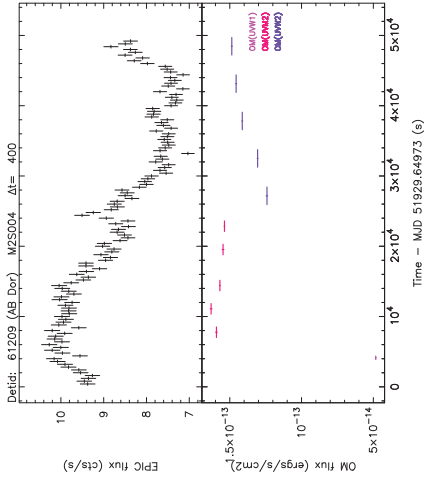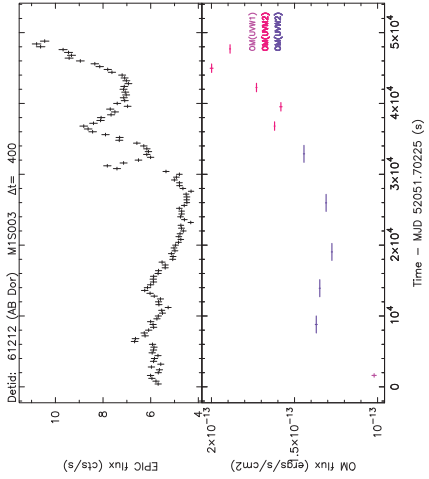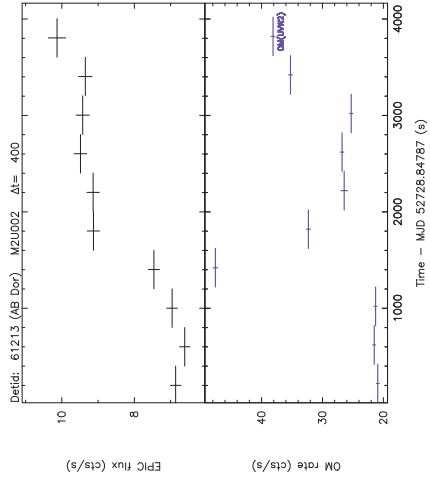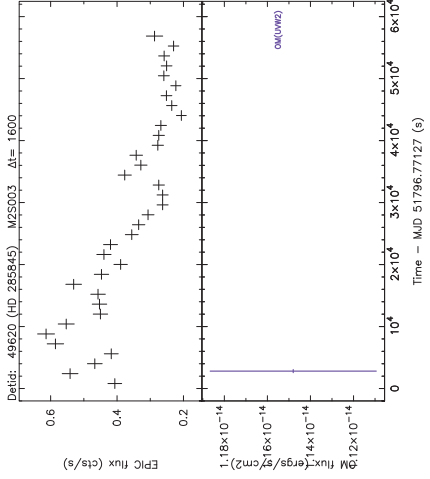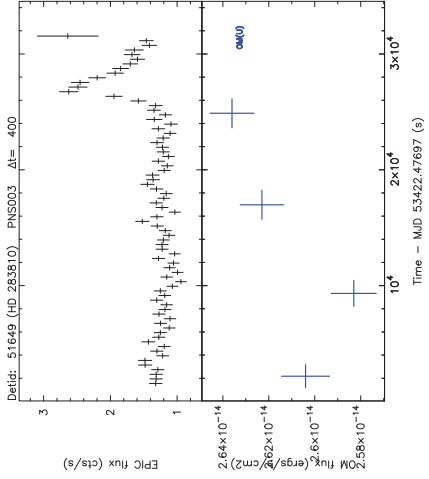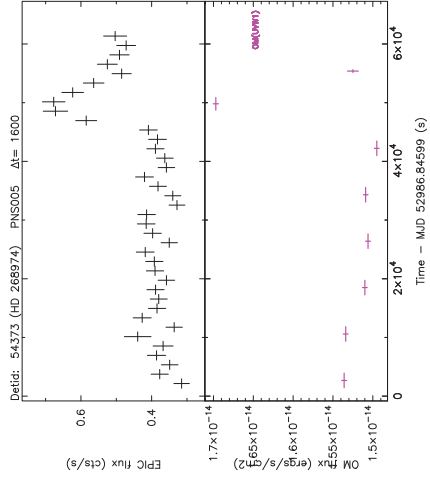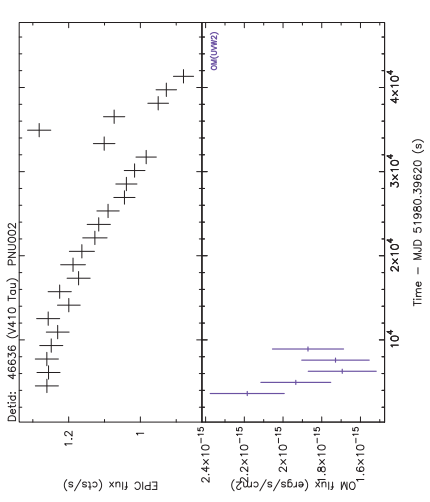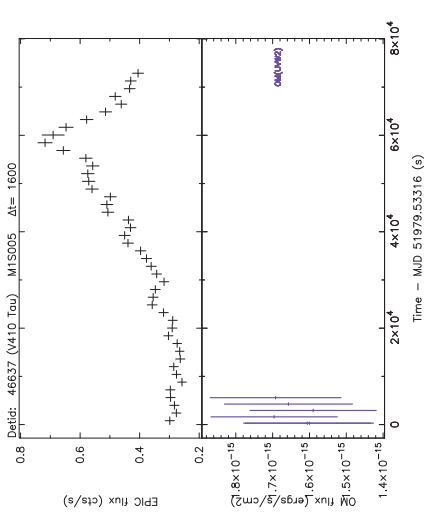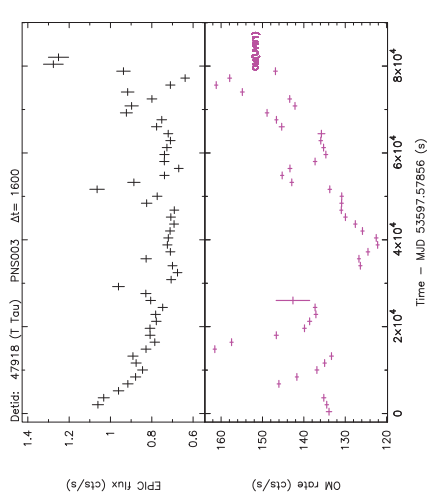

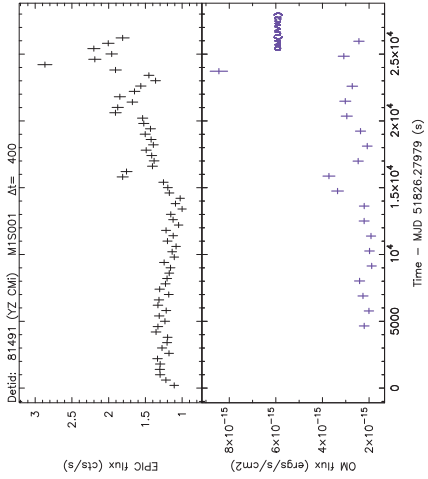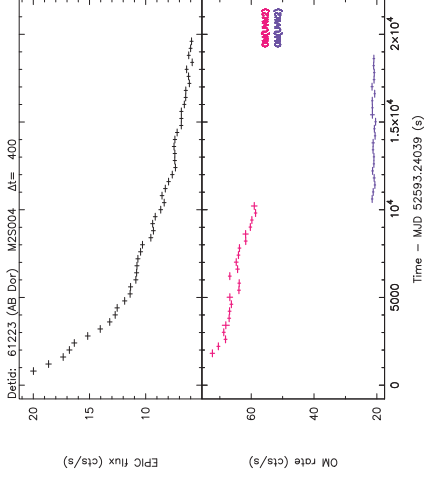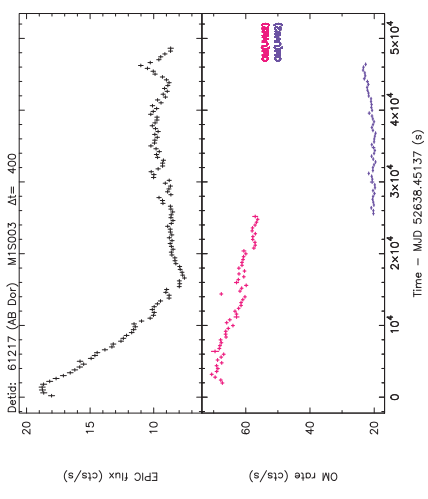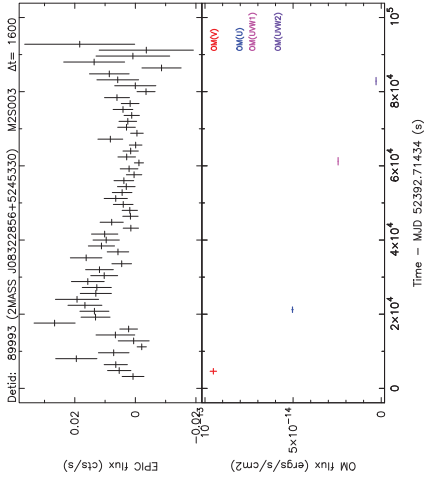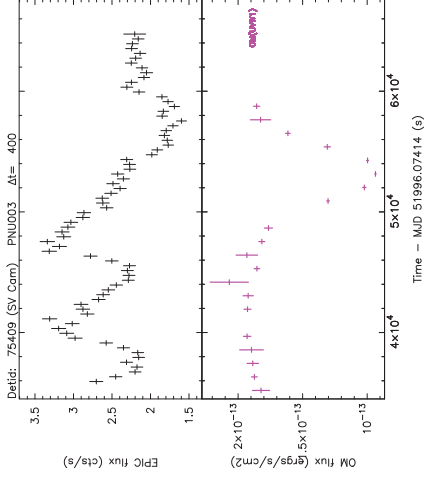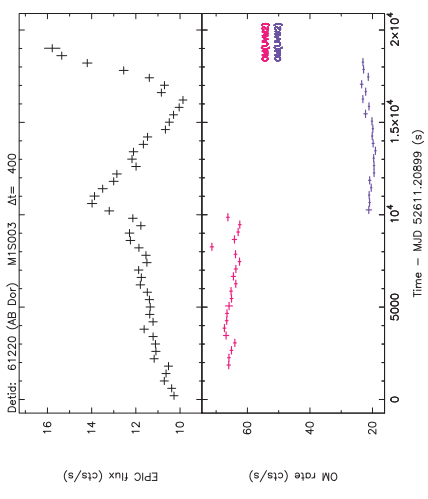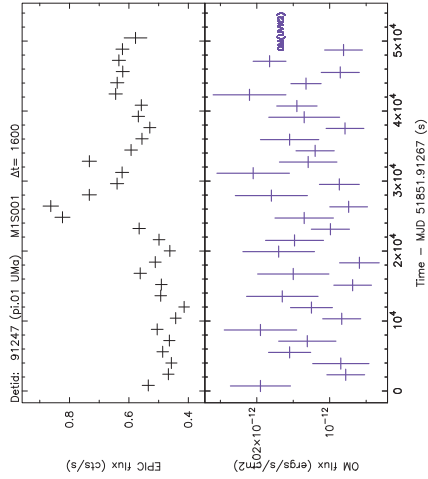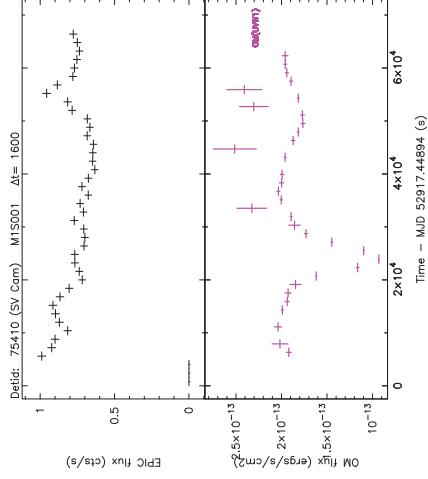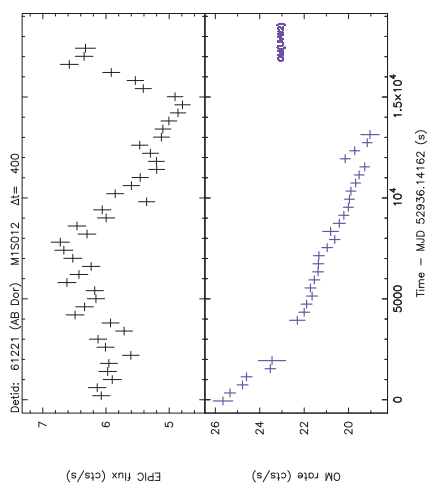

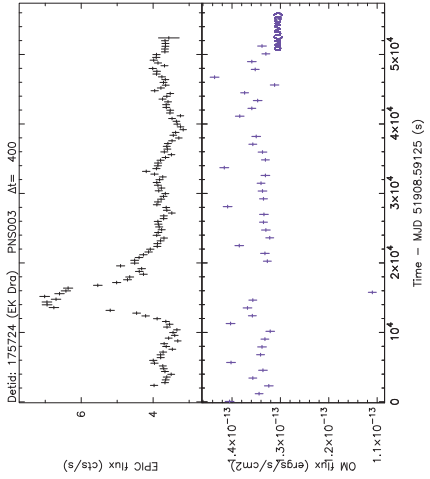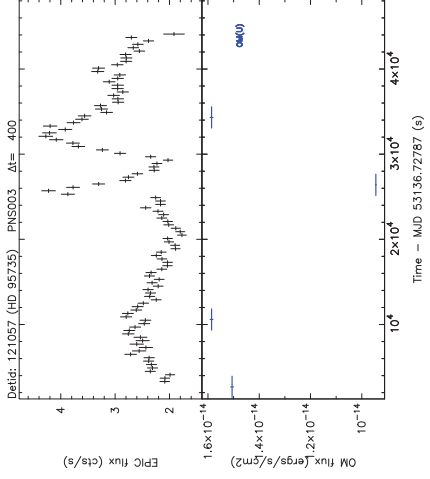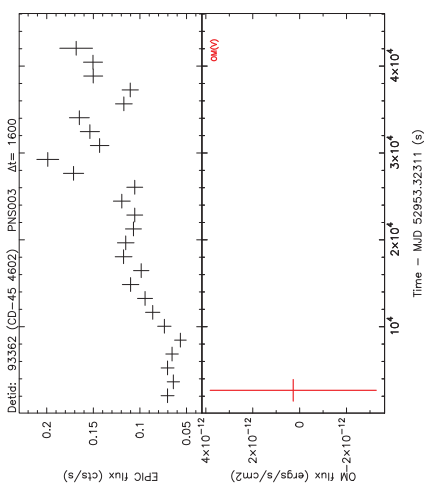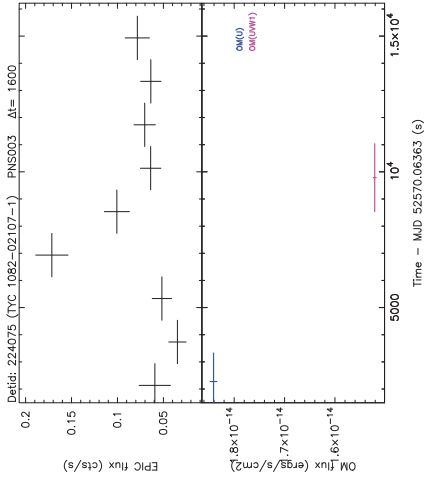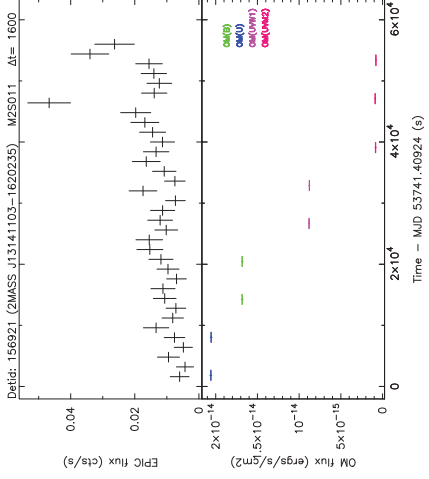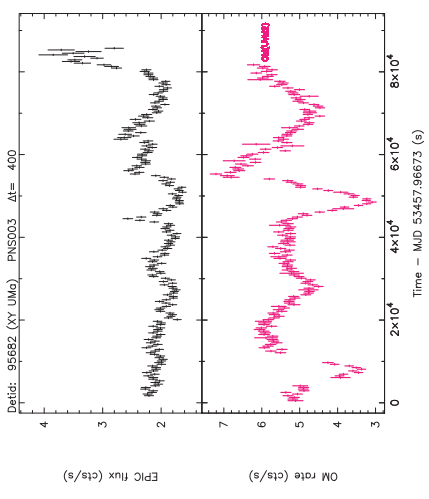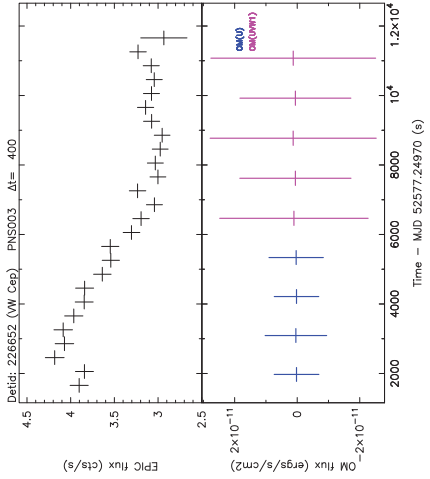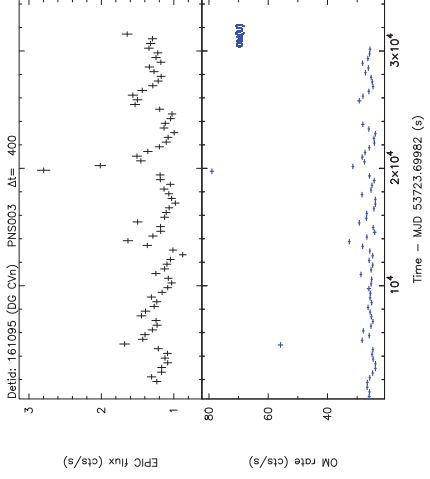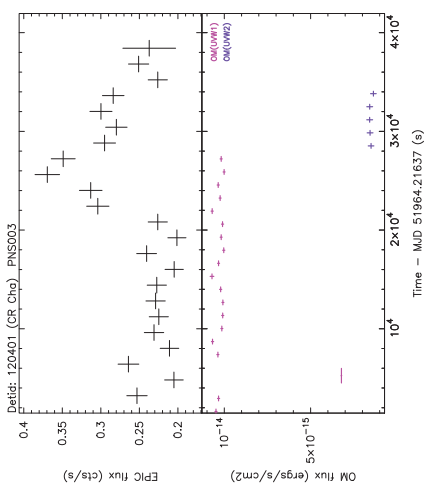

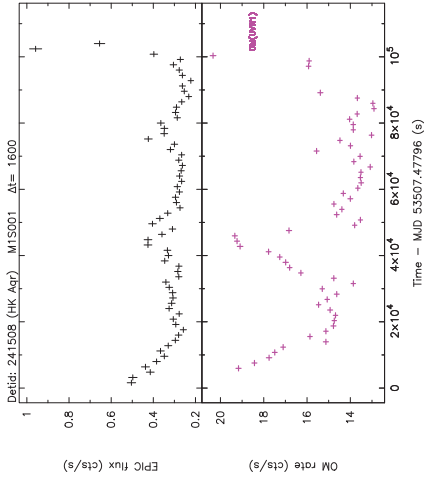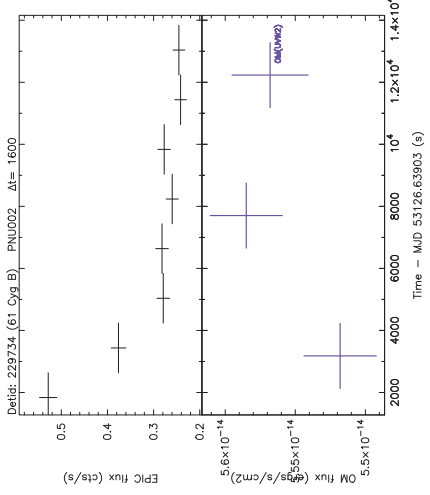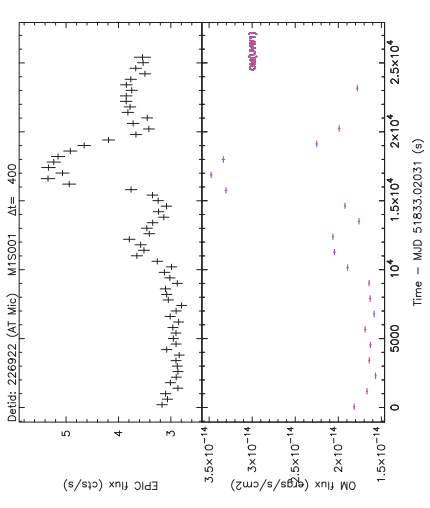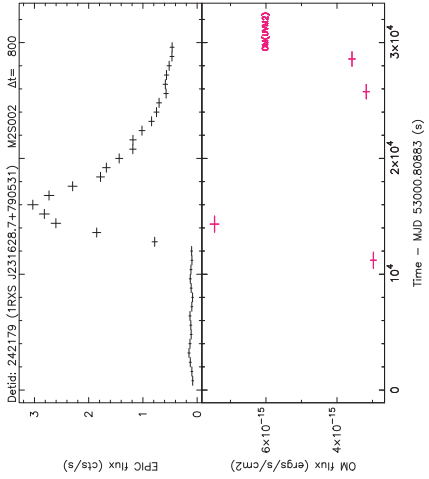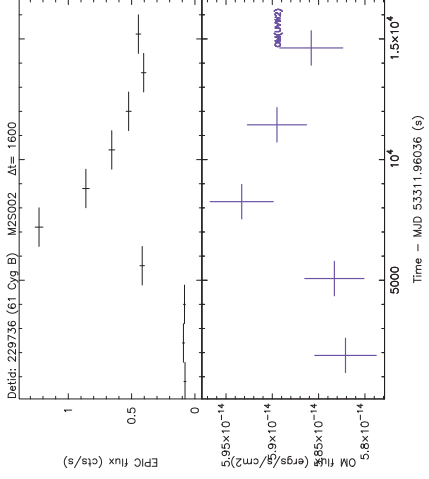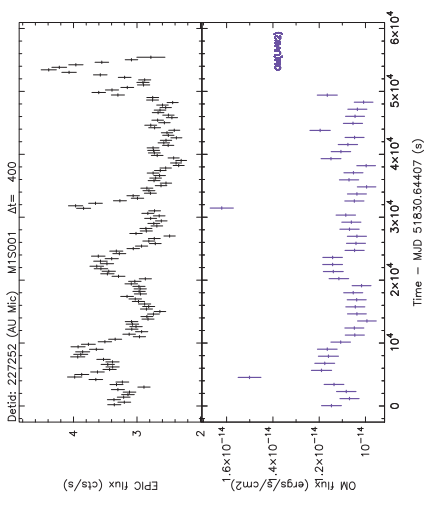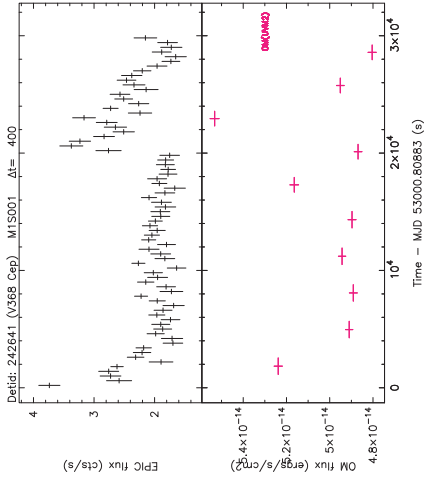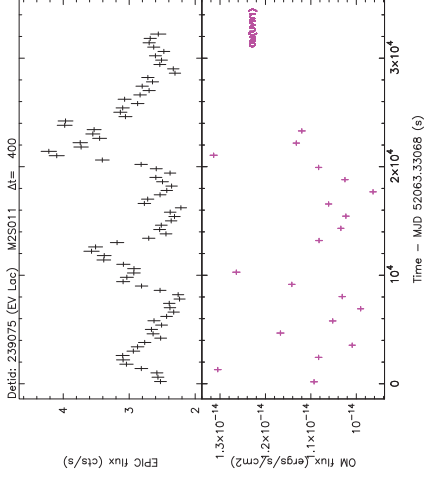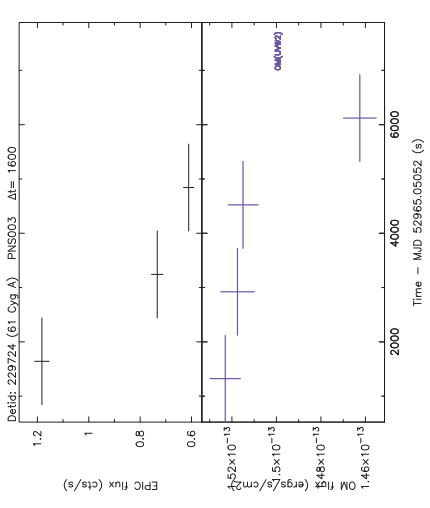

Supplement: Supplementary file 3 [file fig-C.1-CR-OM-lc-All-ElOnly-v02-9perPage.pdf]
